# Supplementary material for: WASP-39b: exo-Saturn with patchy cloud composition, moderate metallicity, and underdepleted S/O
Source: arXiv:2301.08492 source file (2025-12-02)

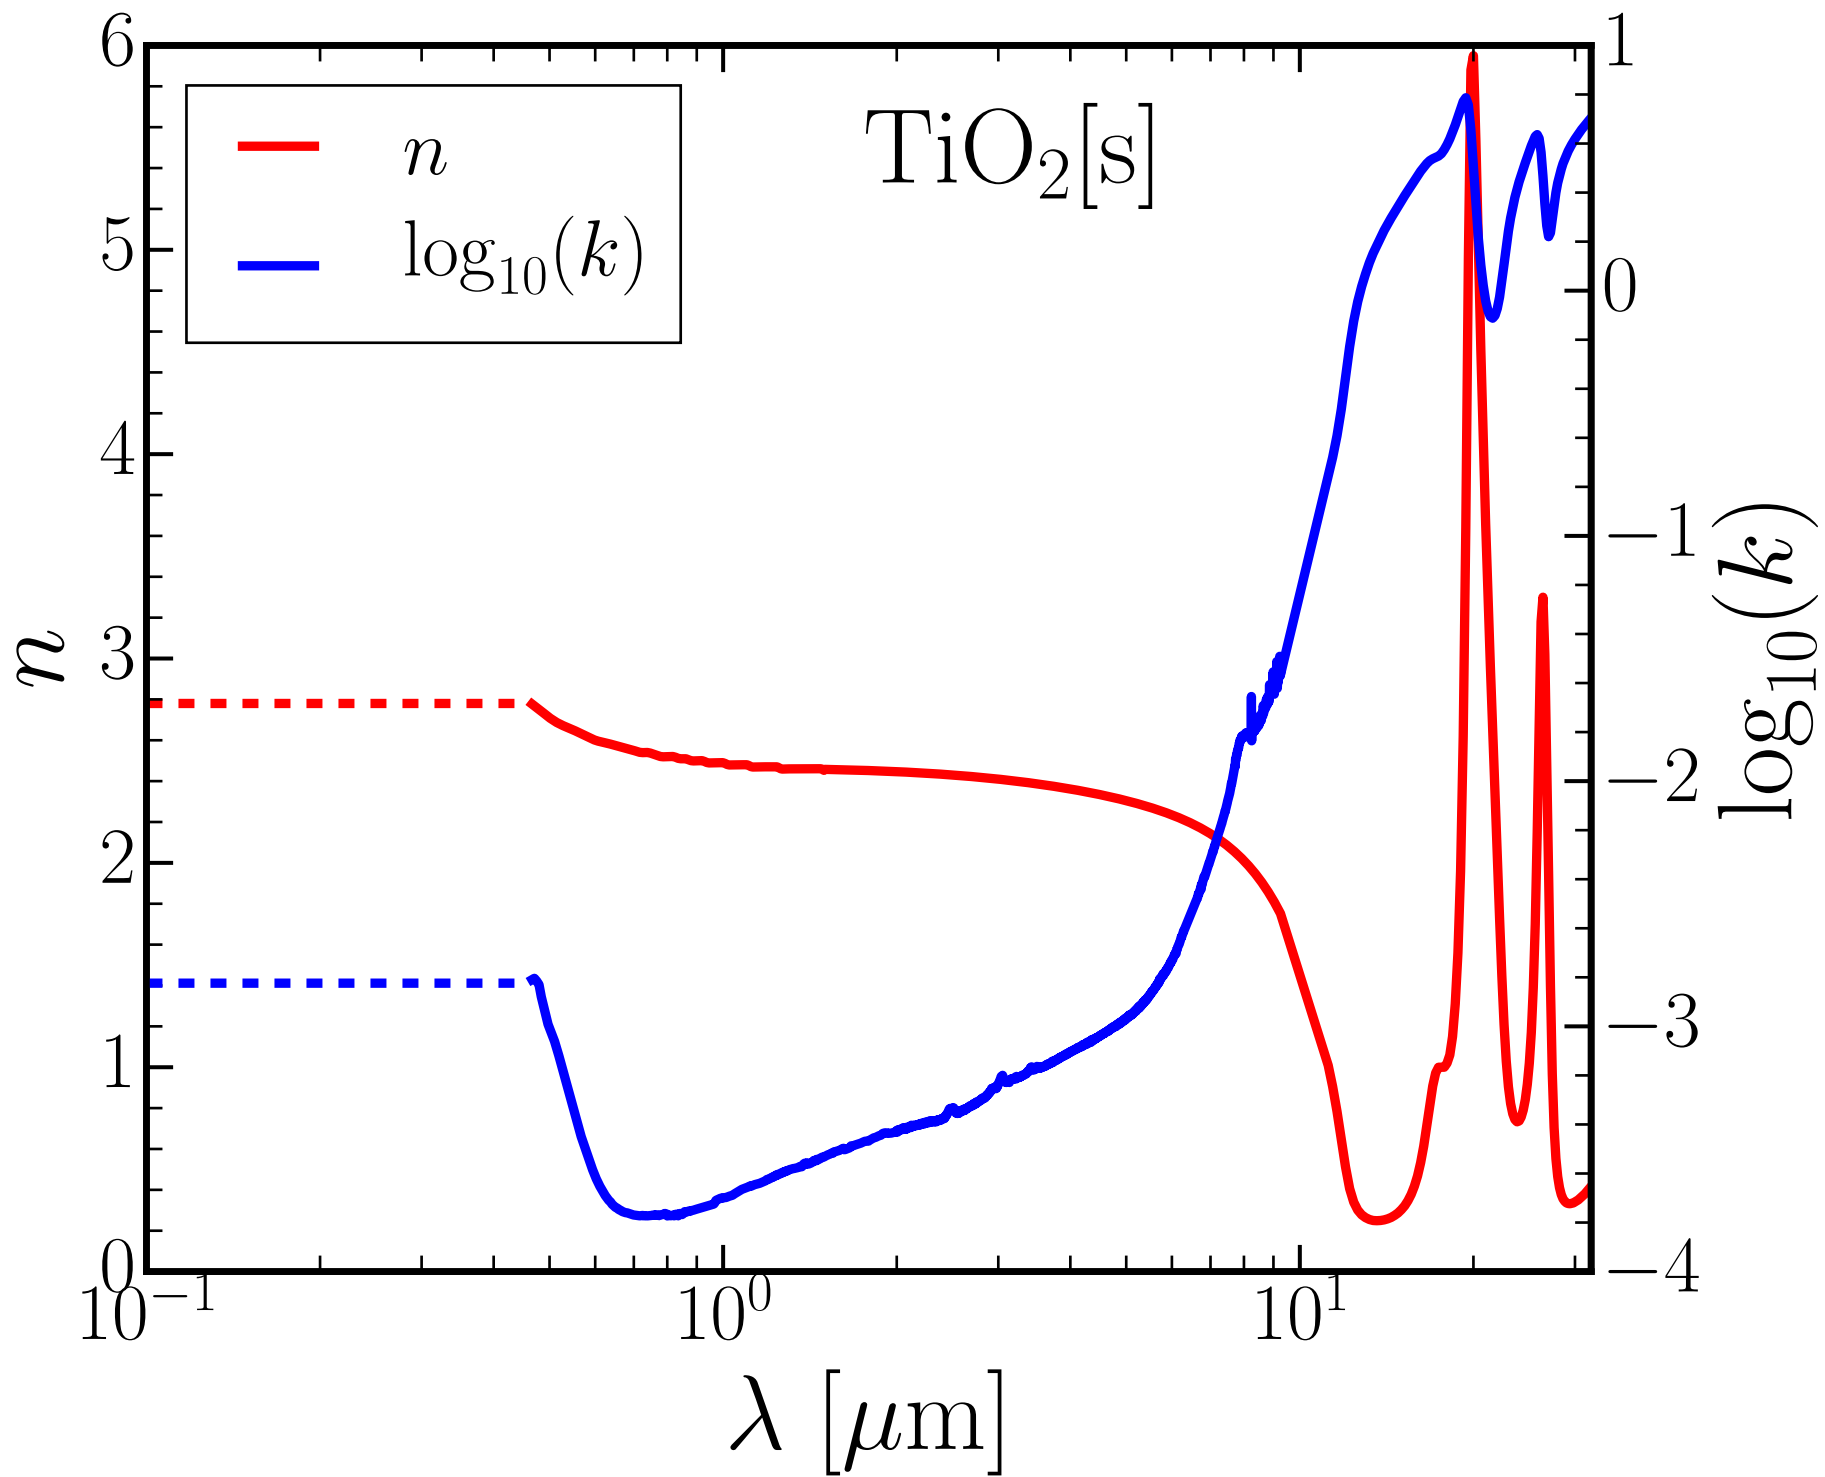

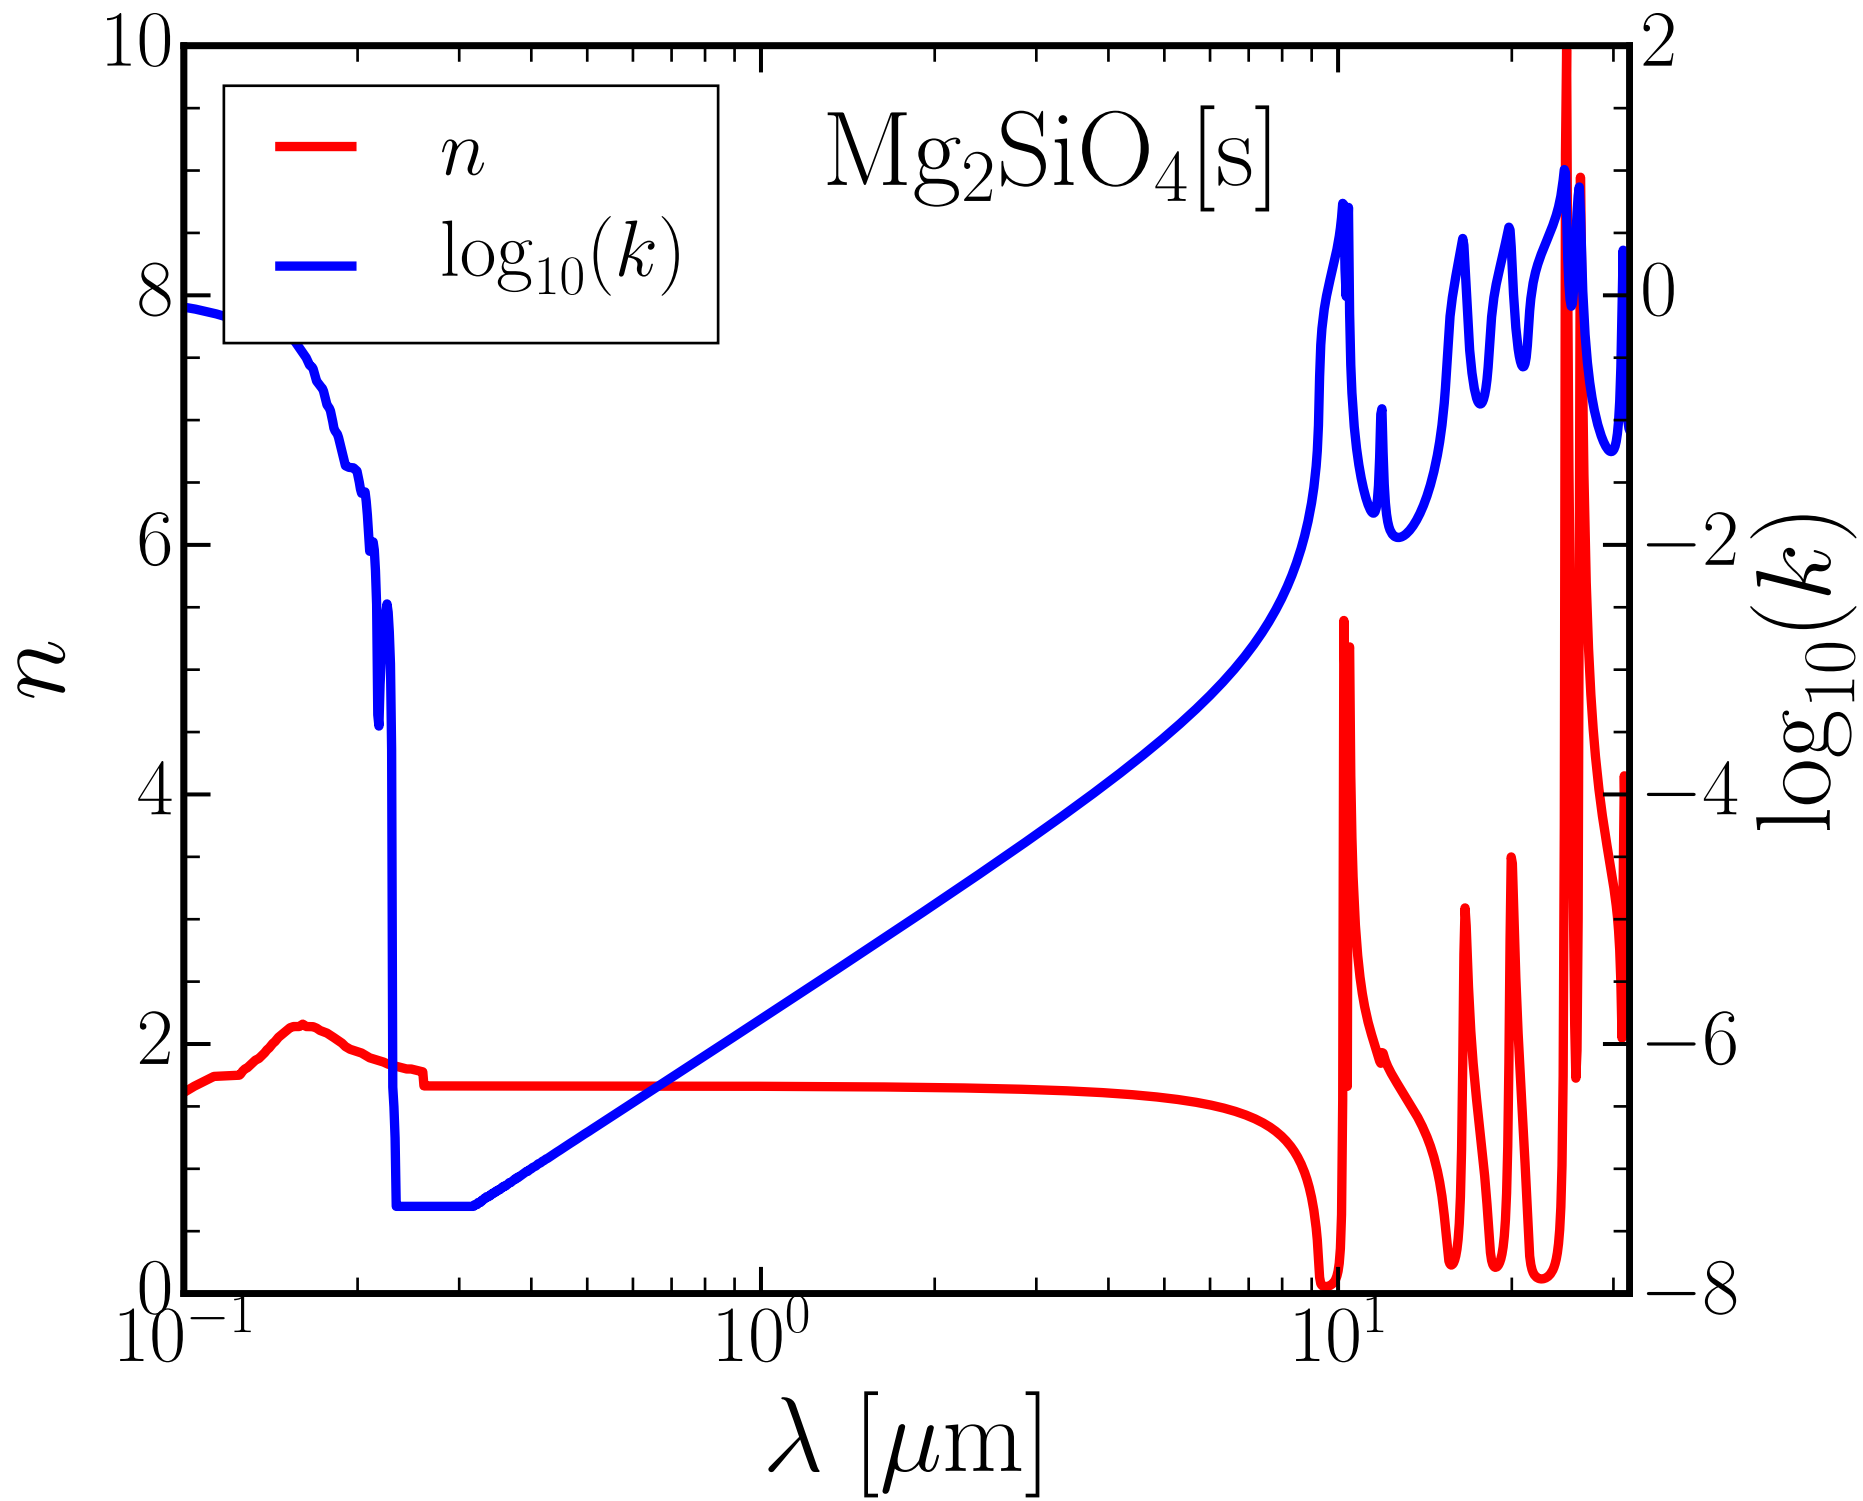

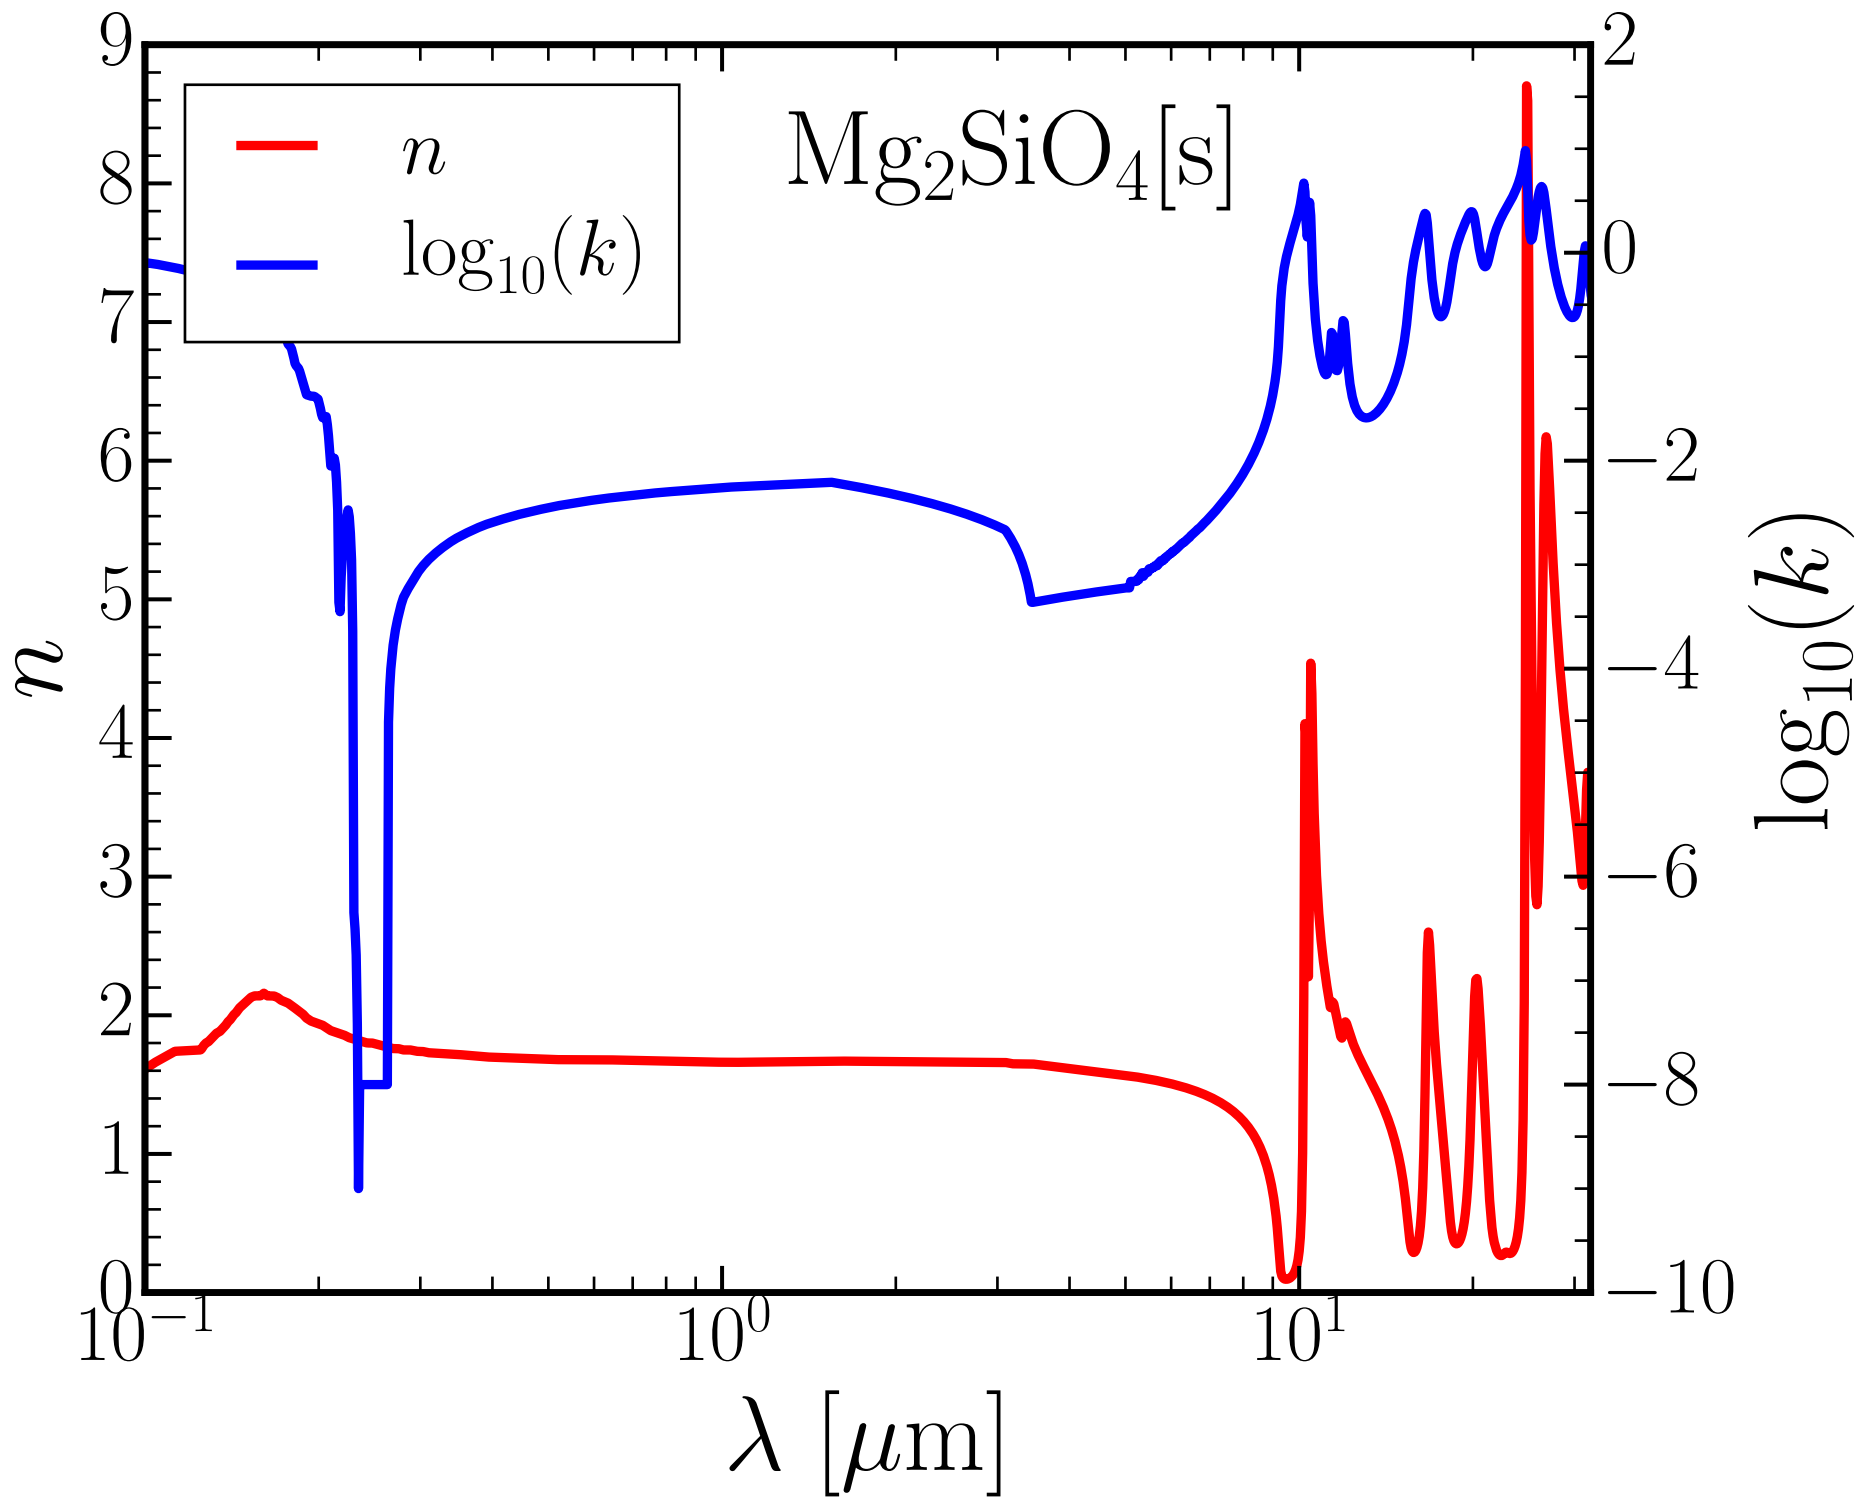

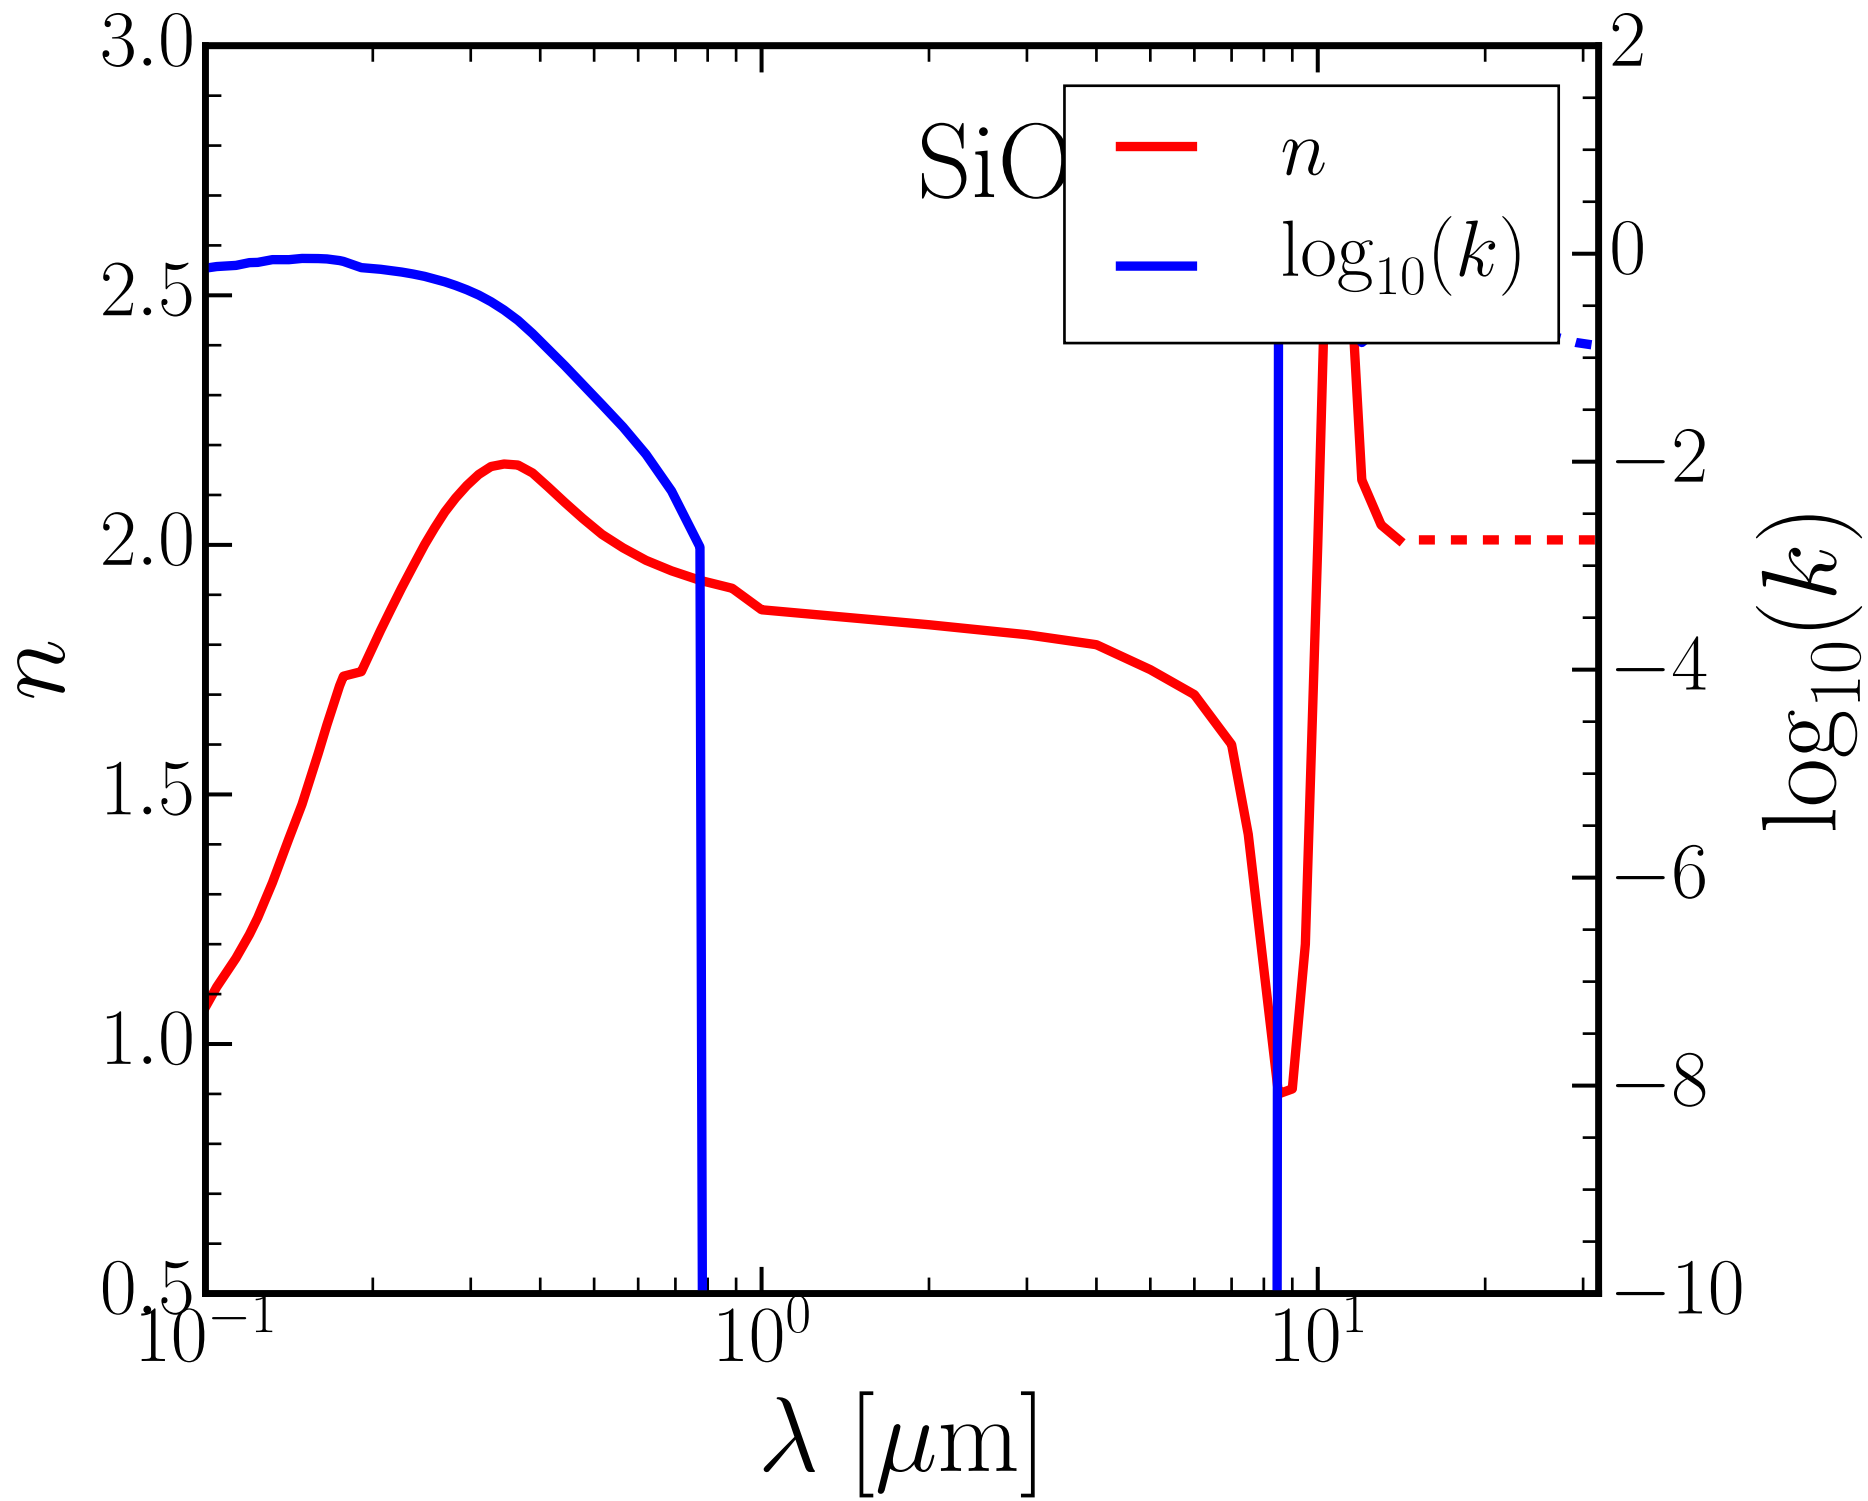

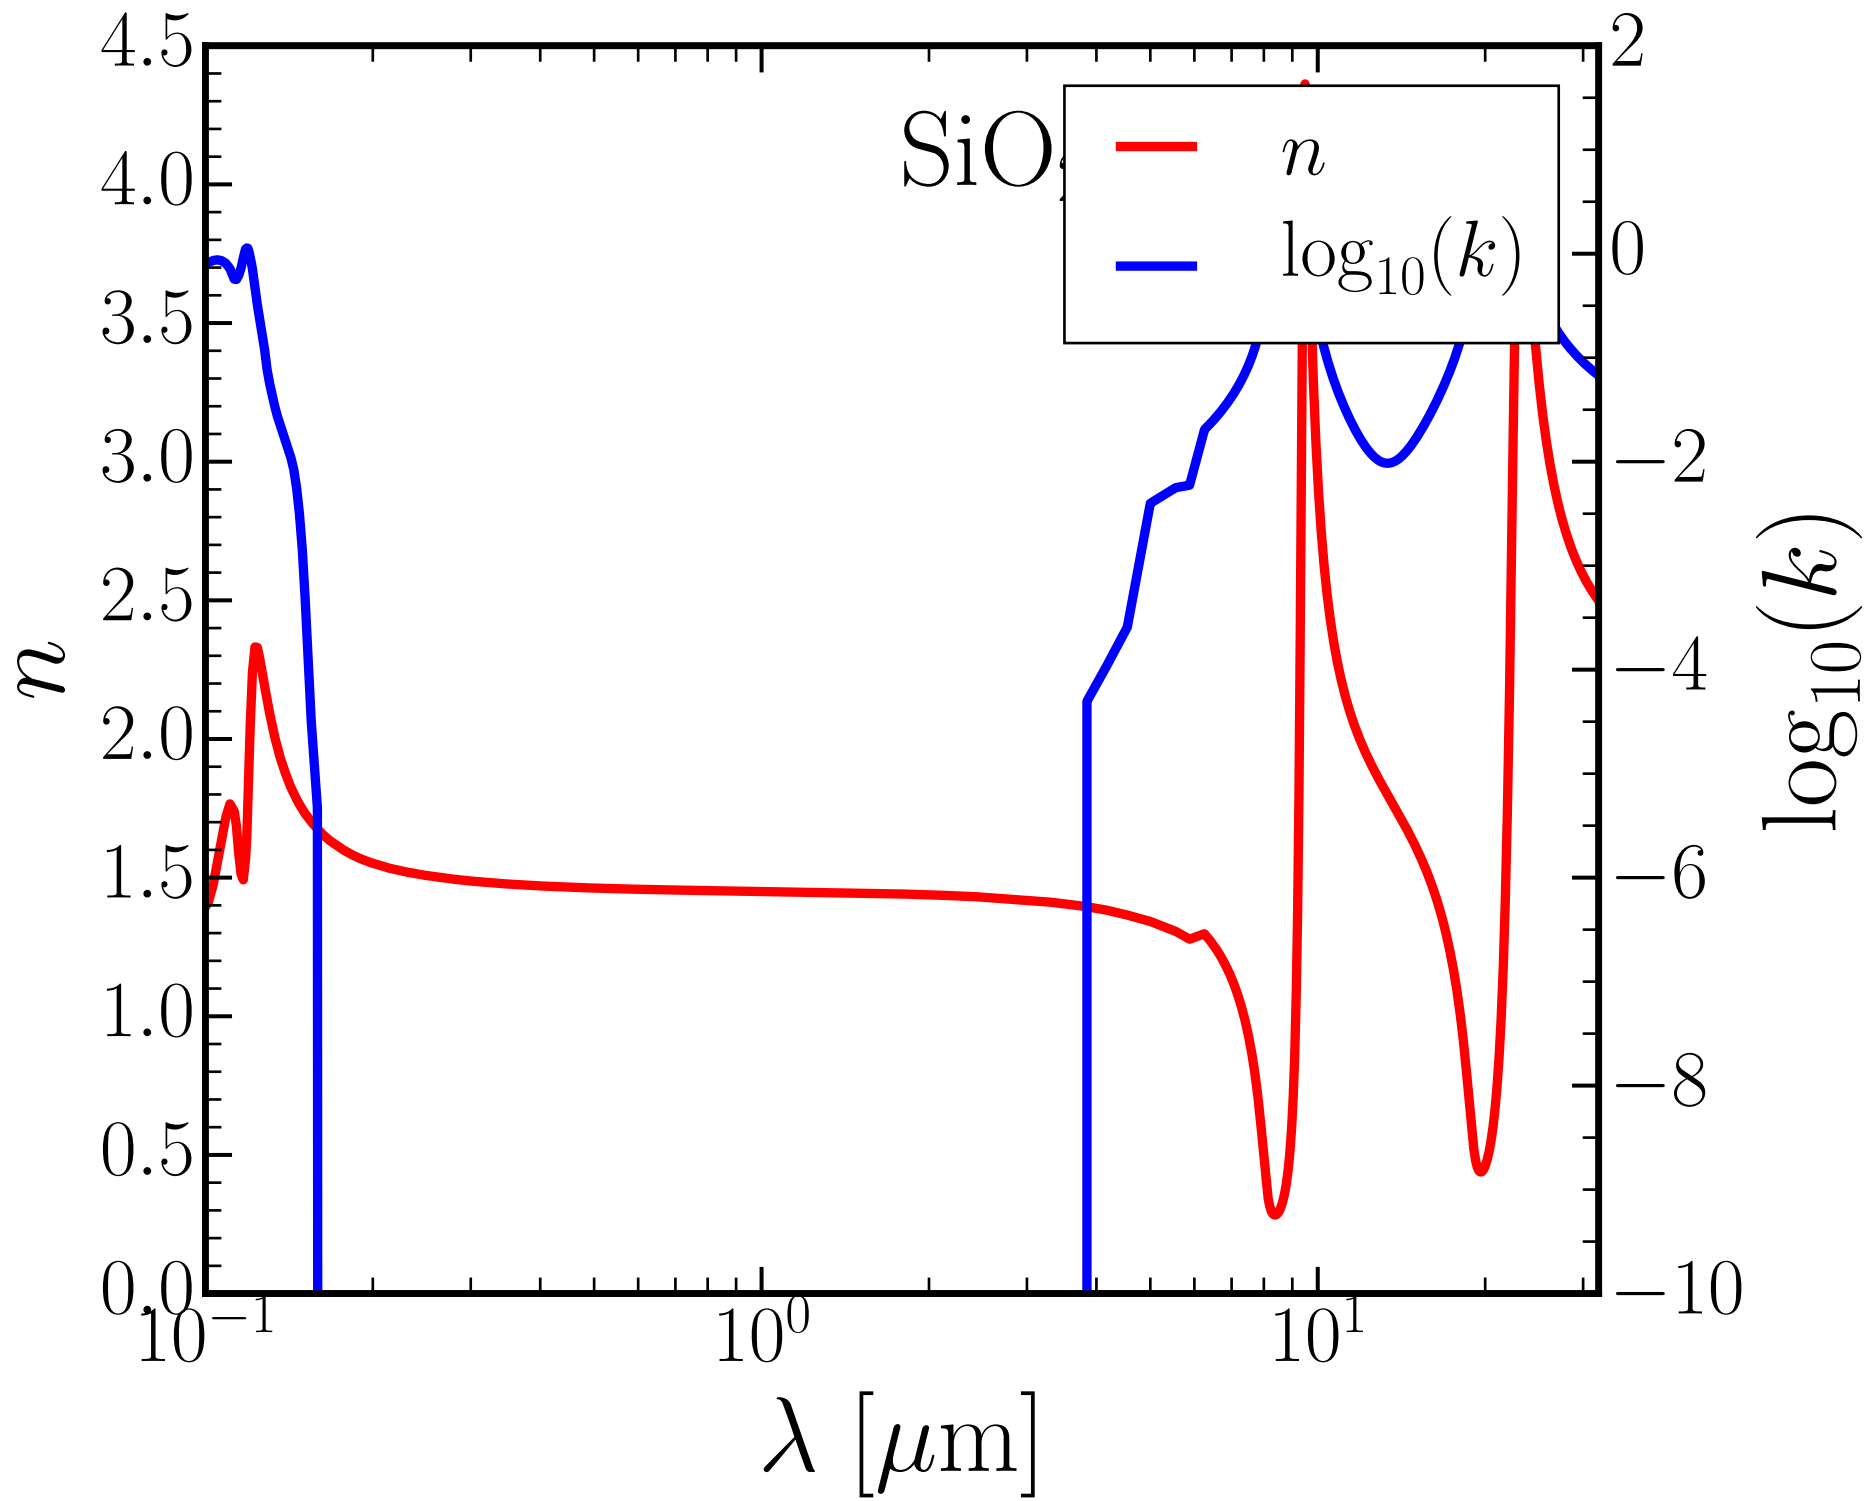

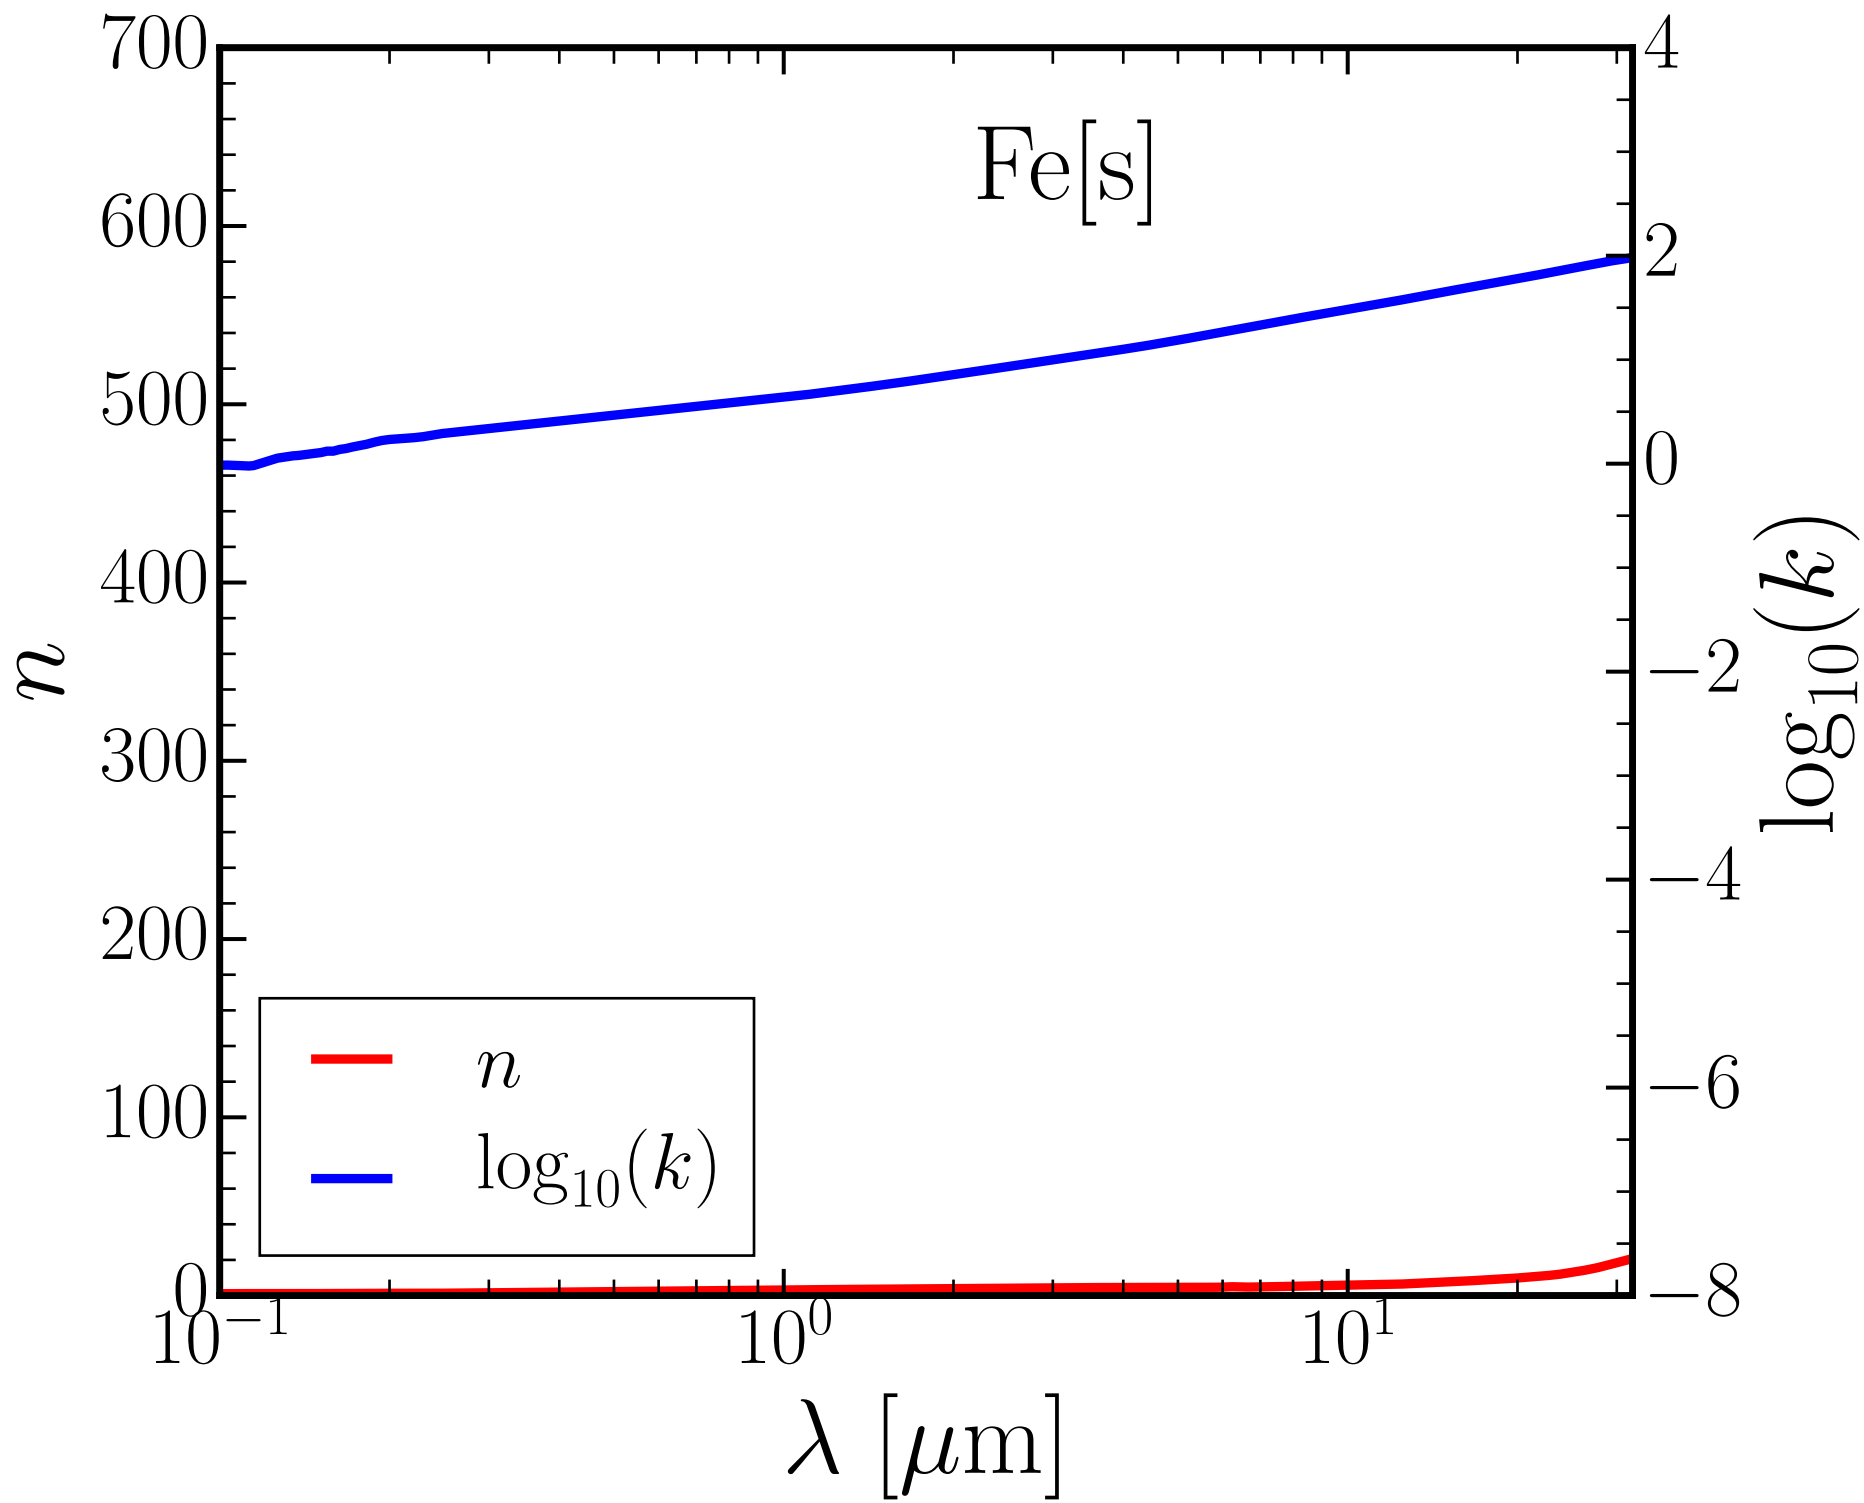

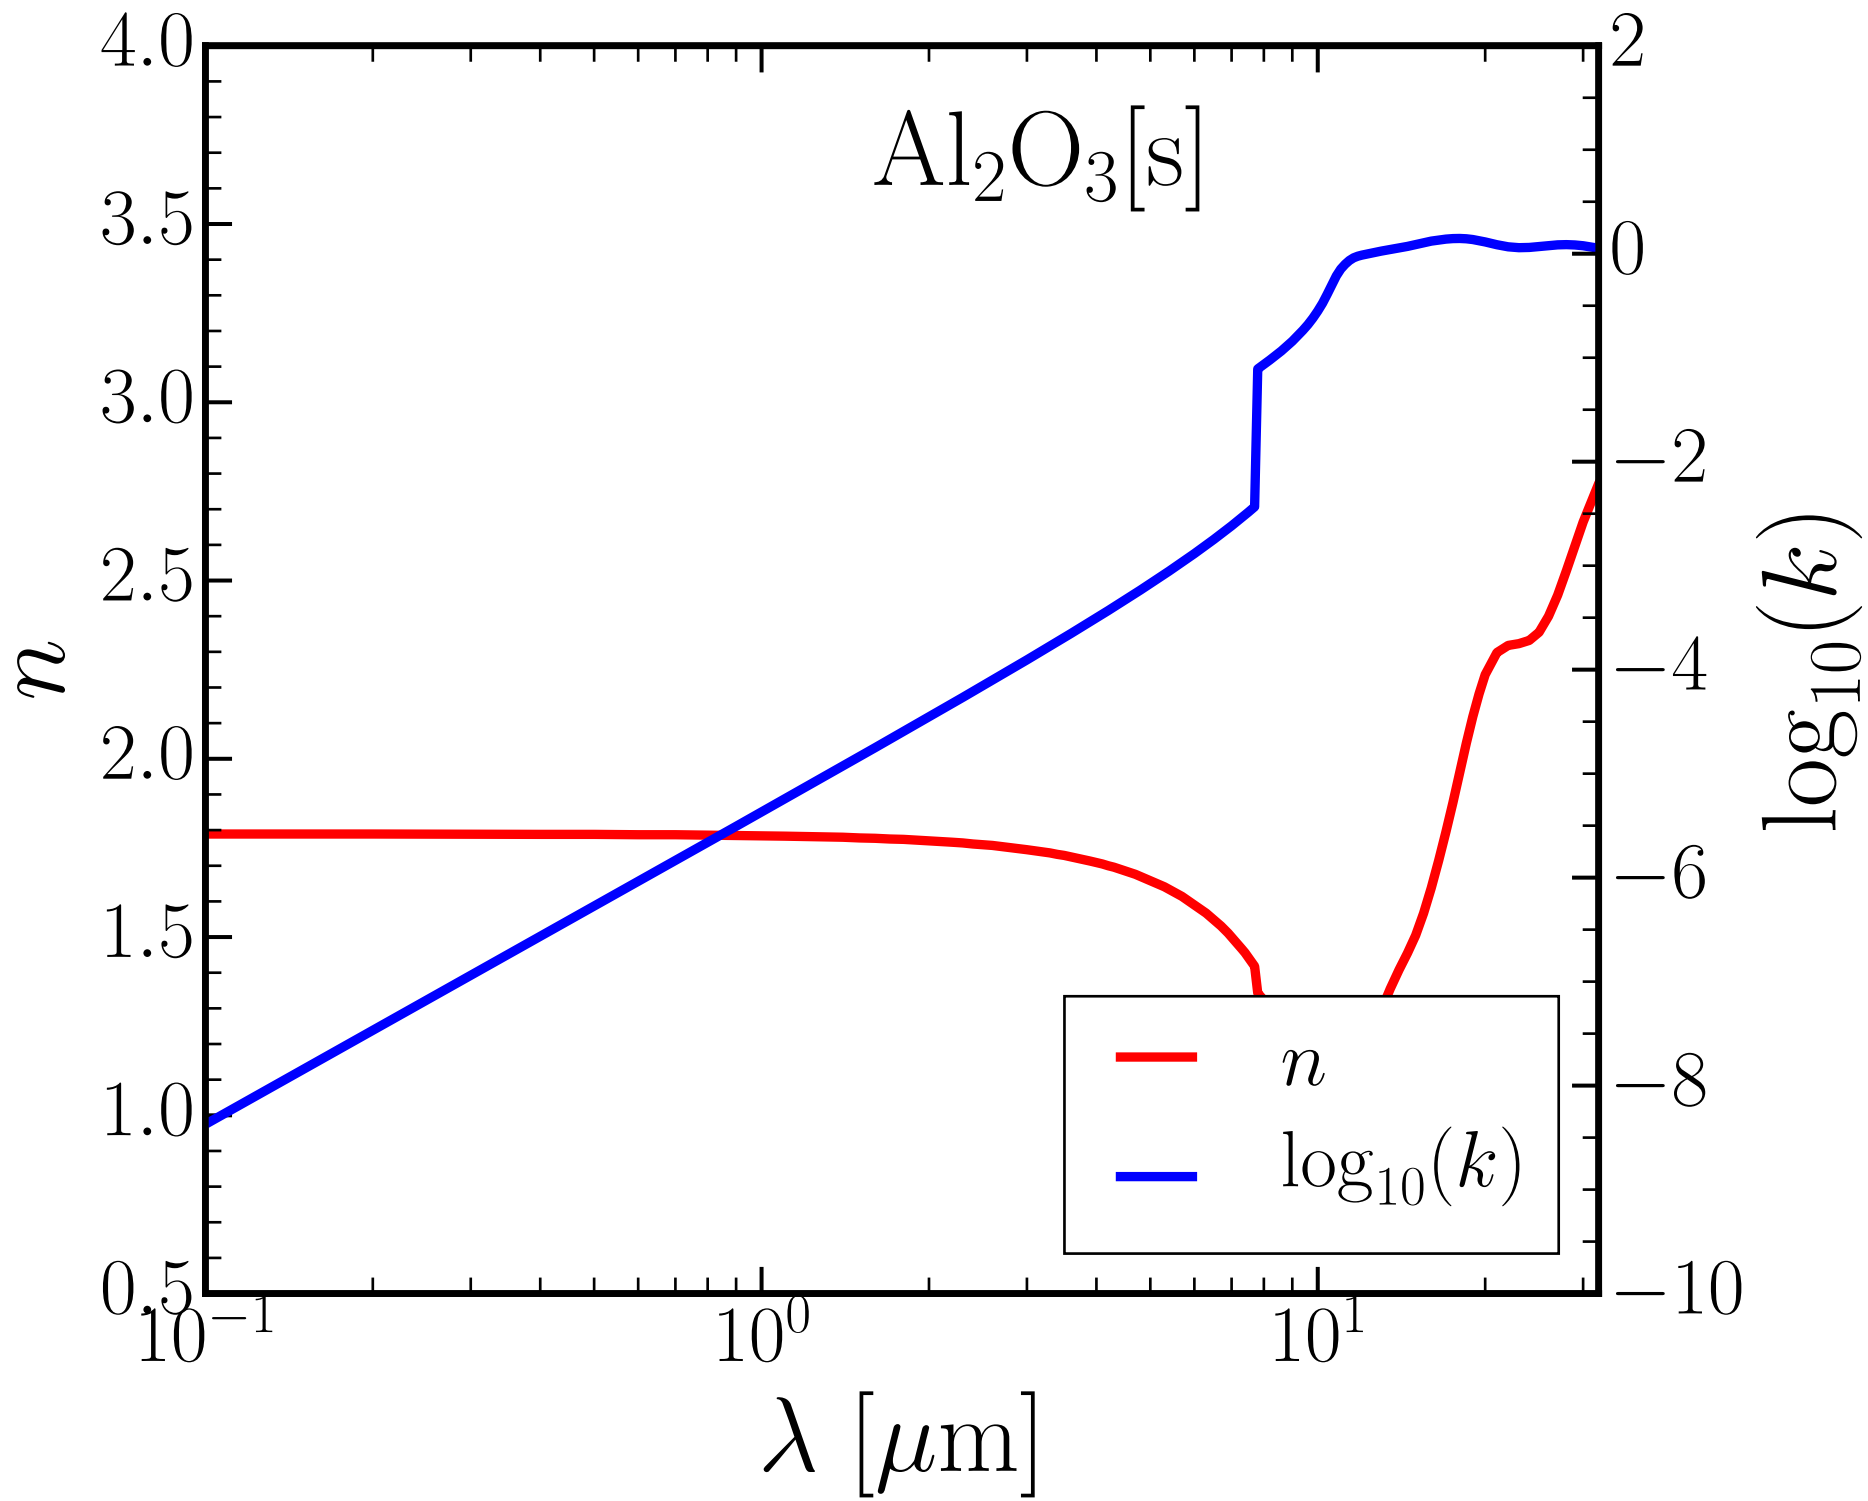

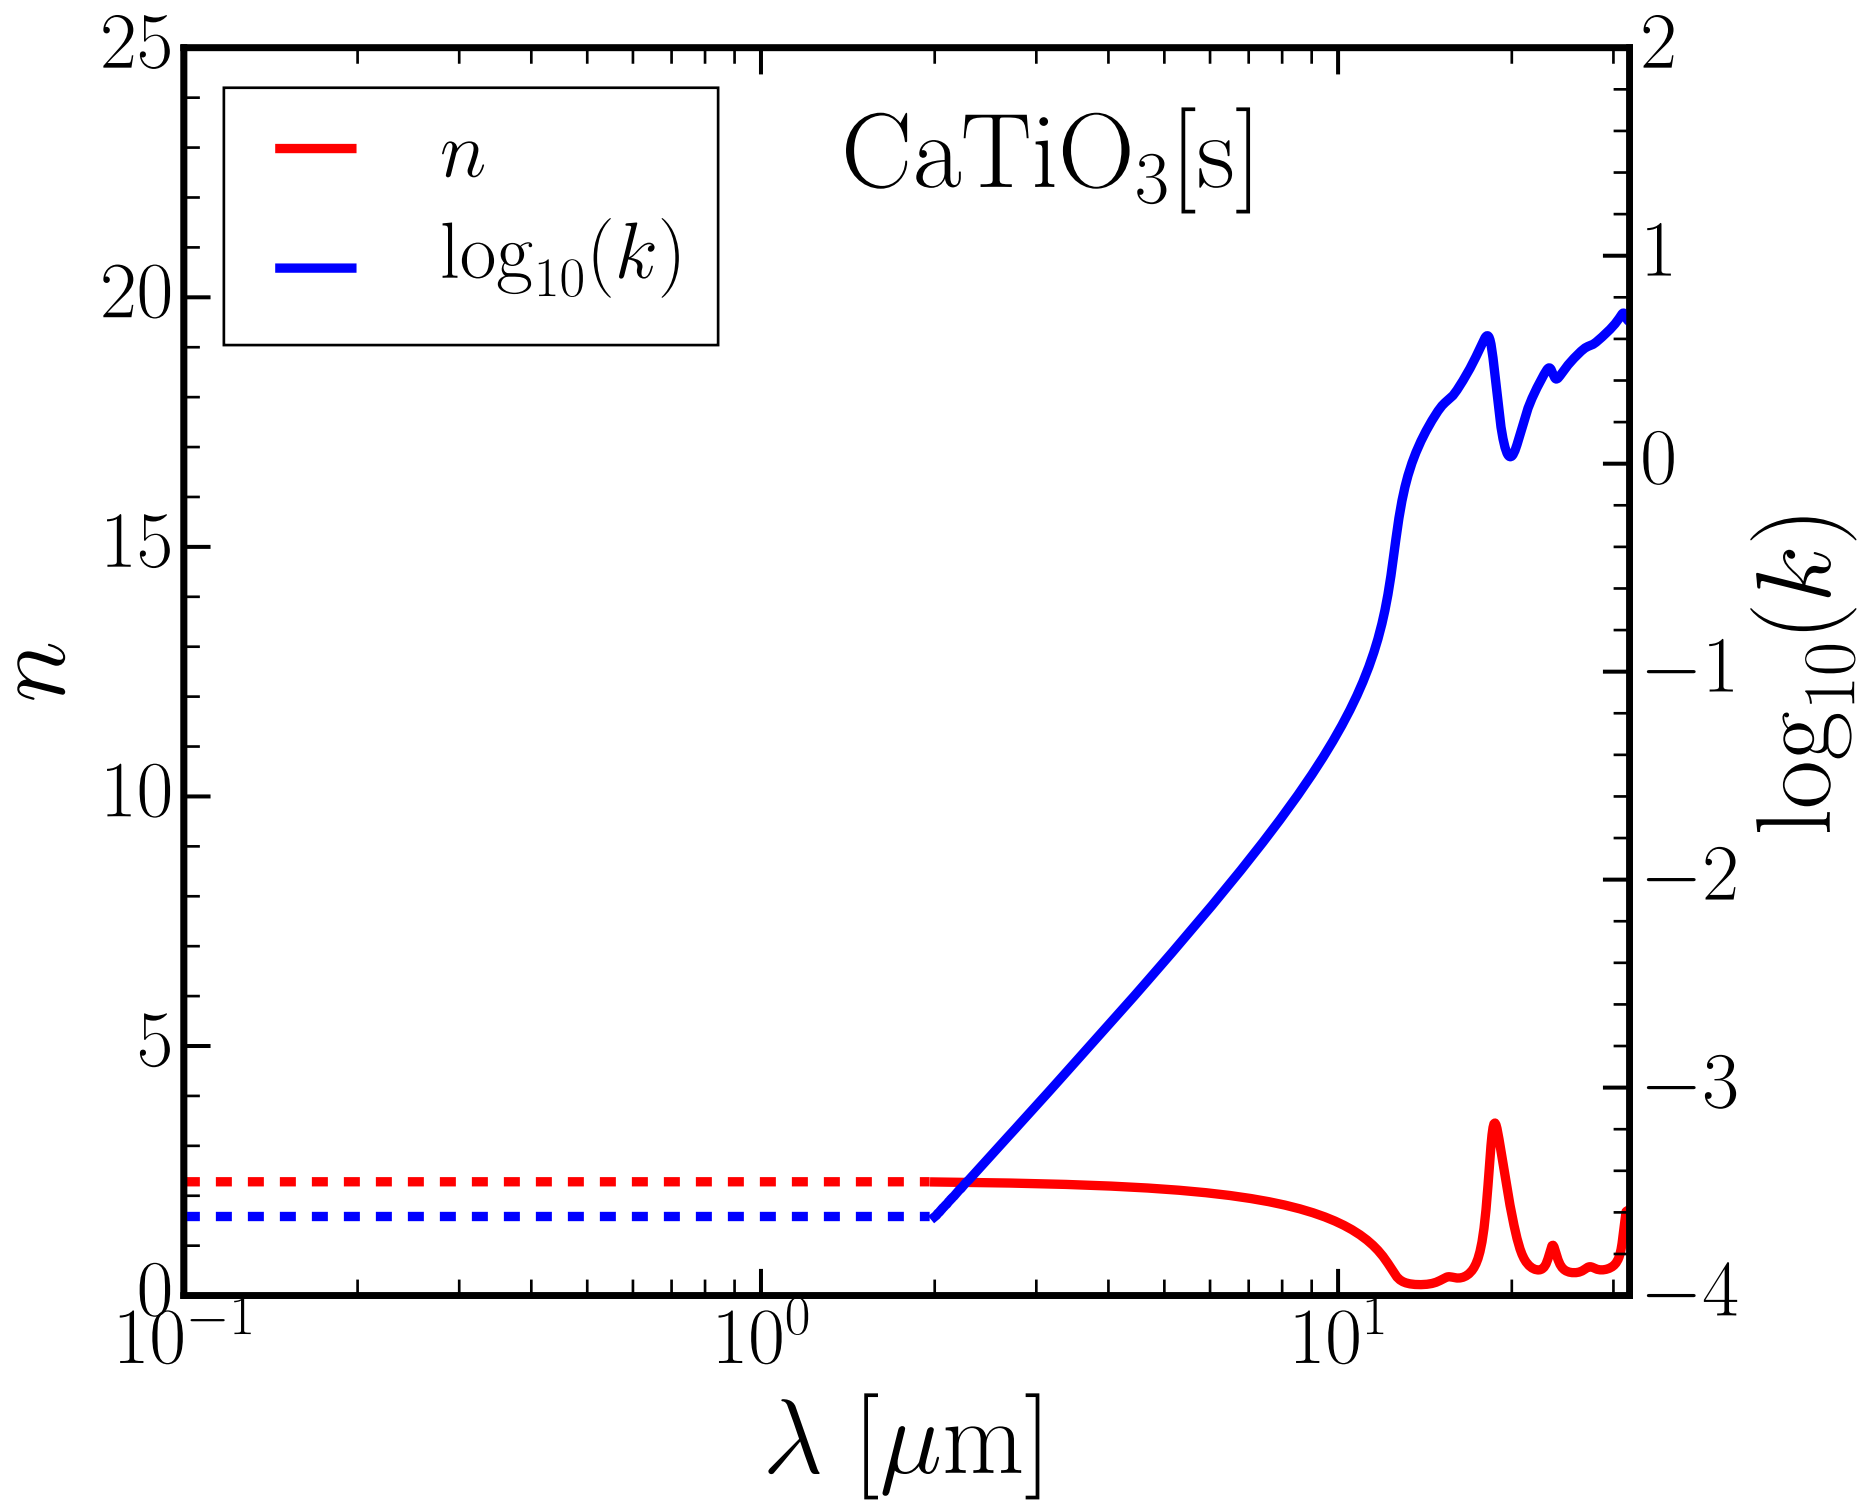



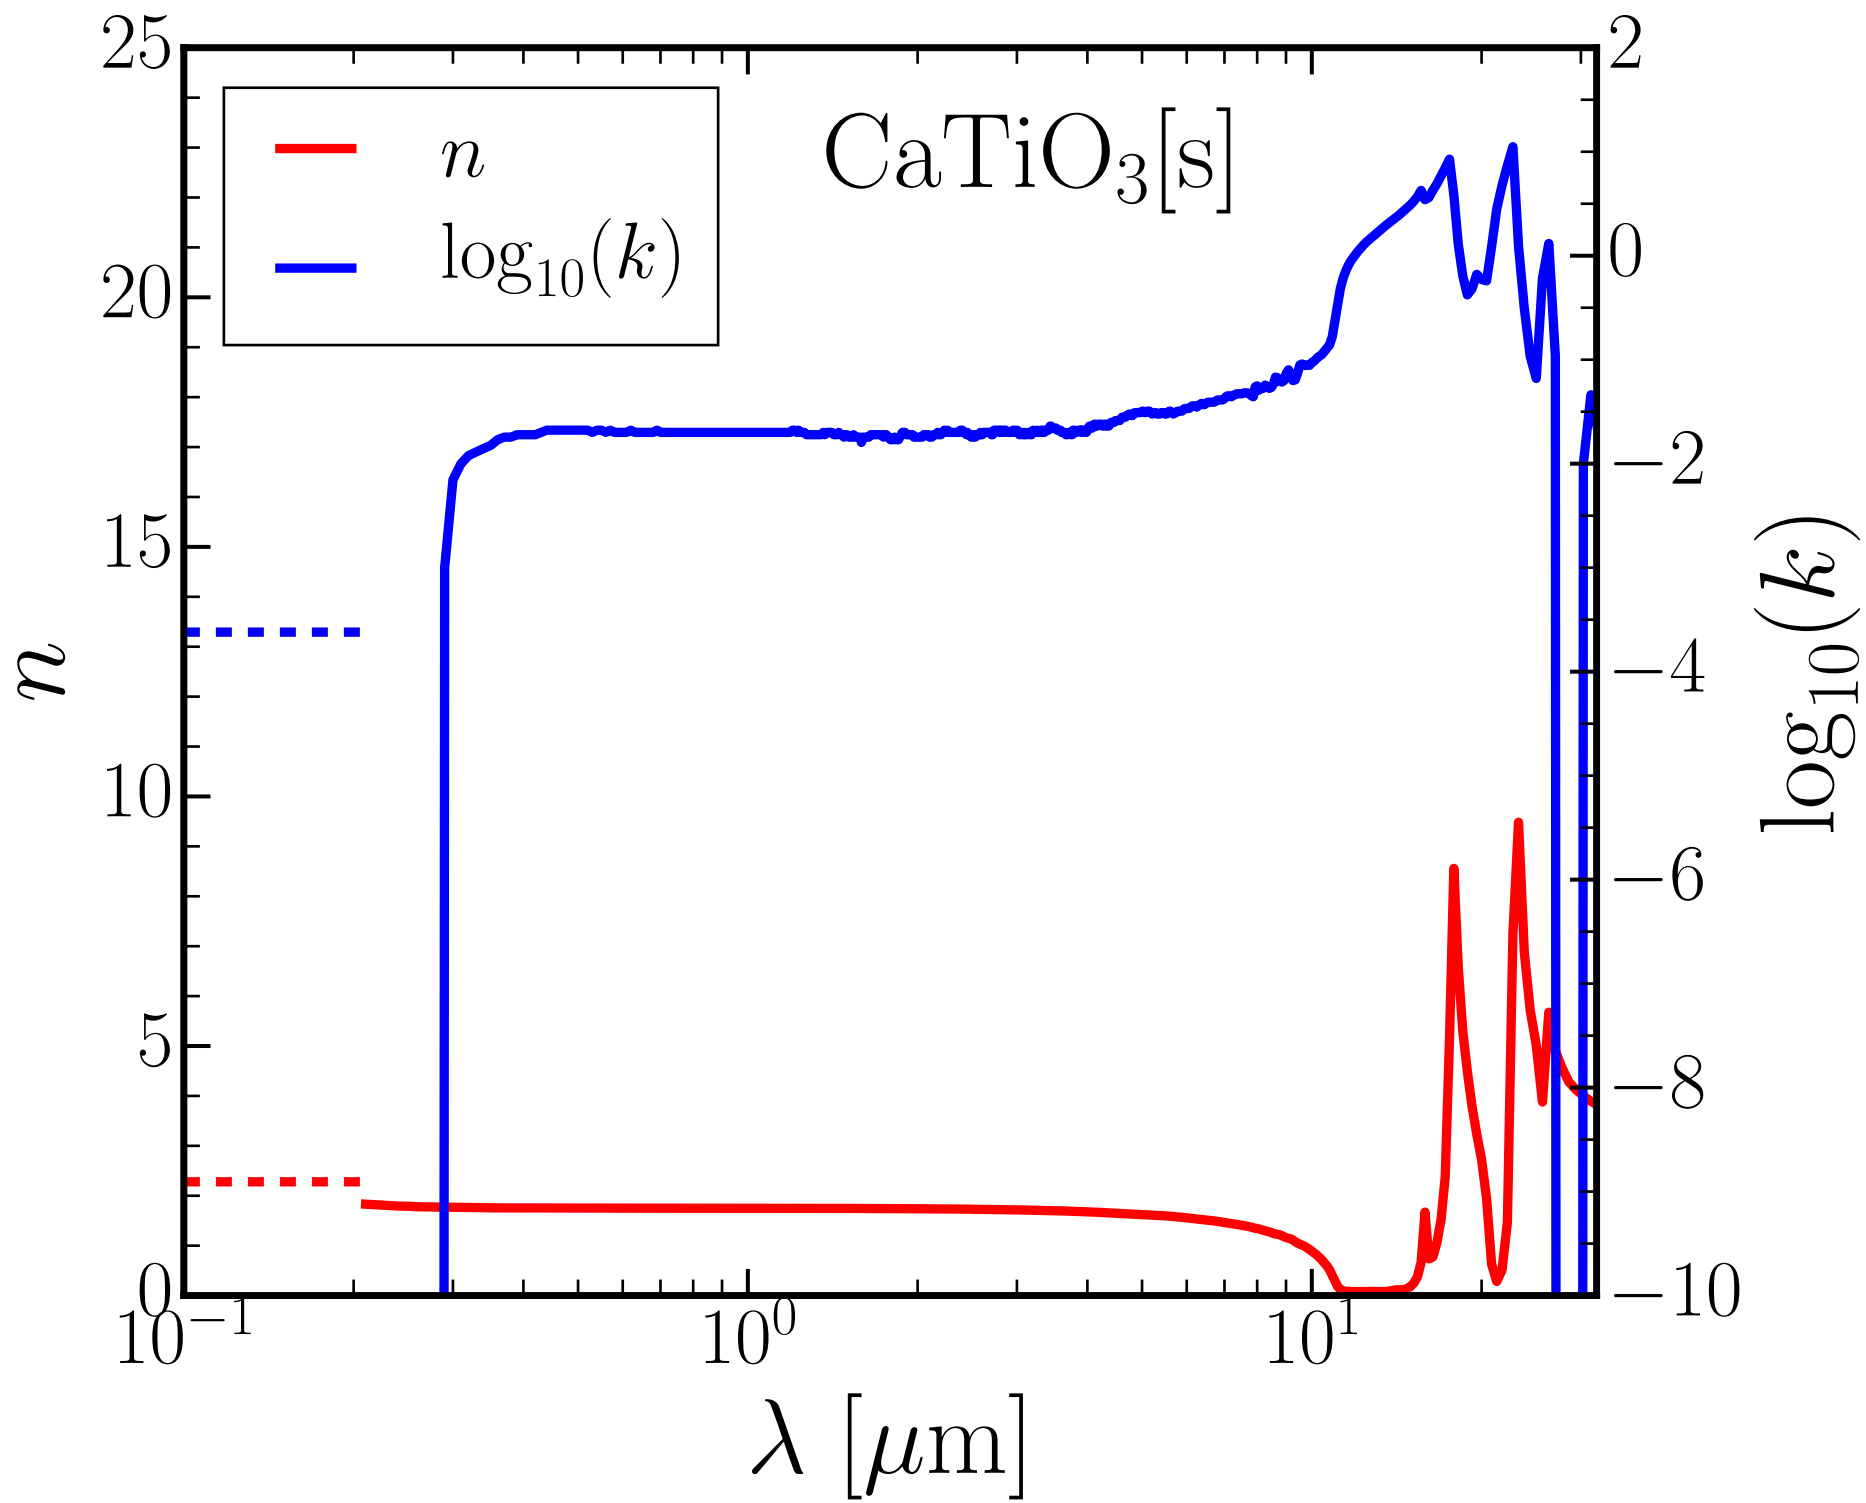

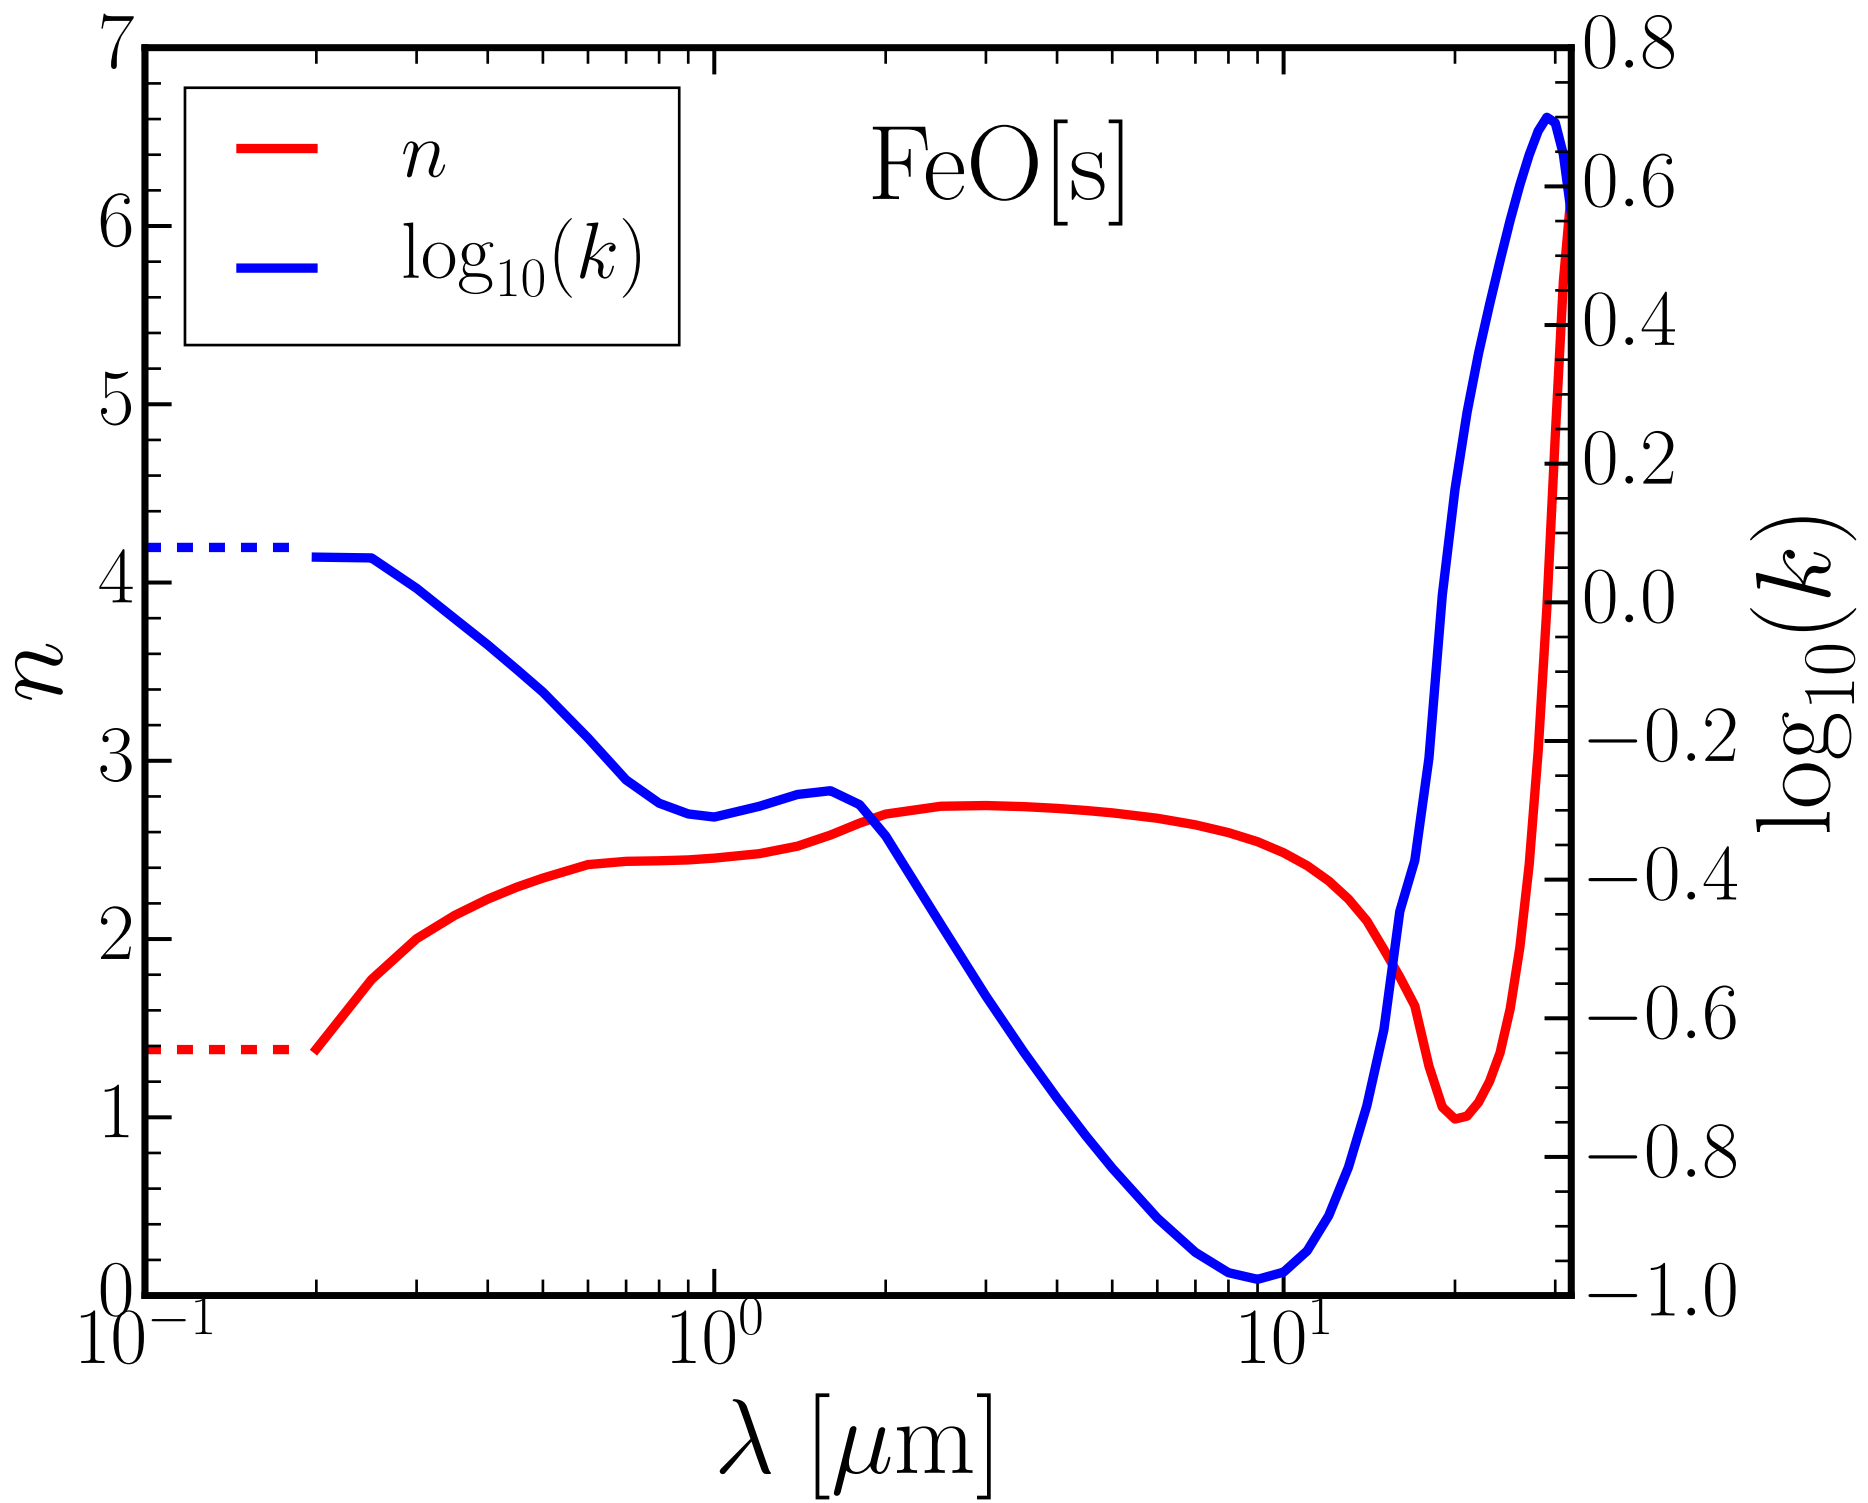

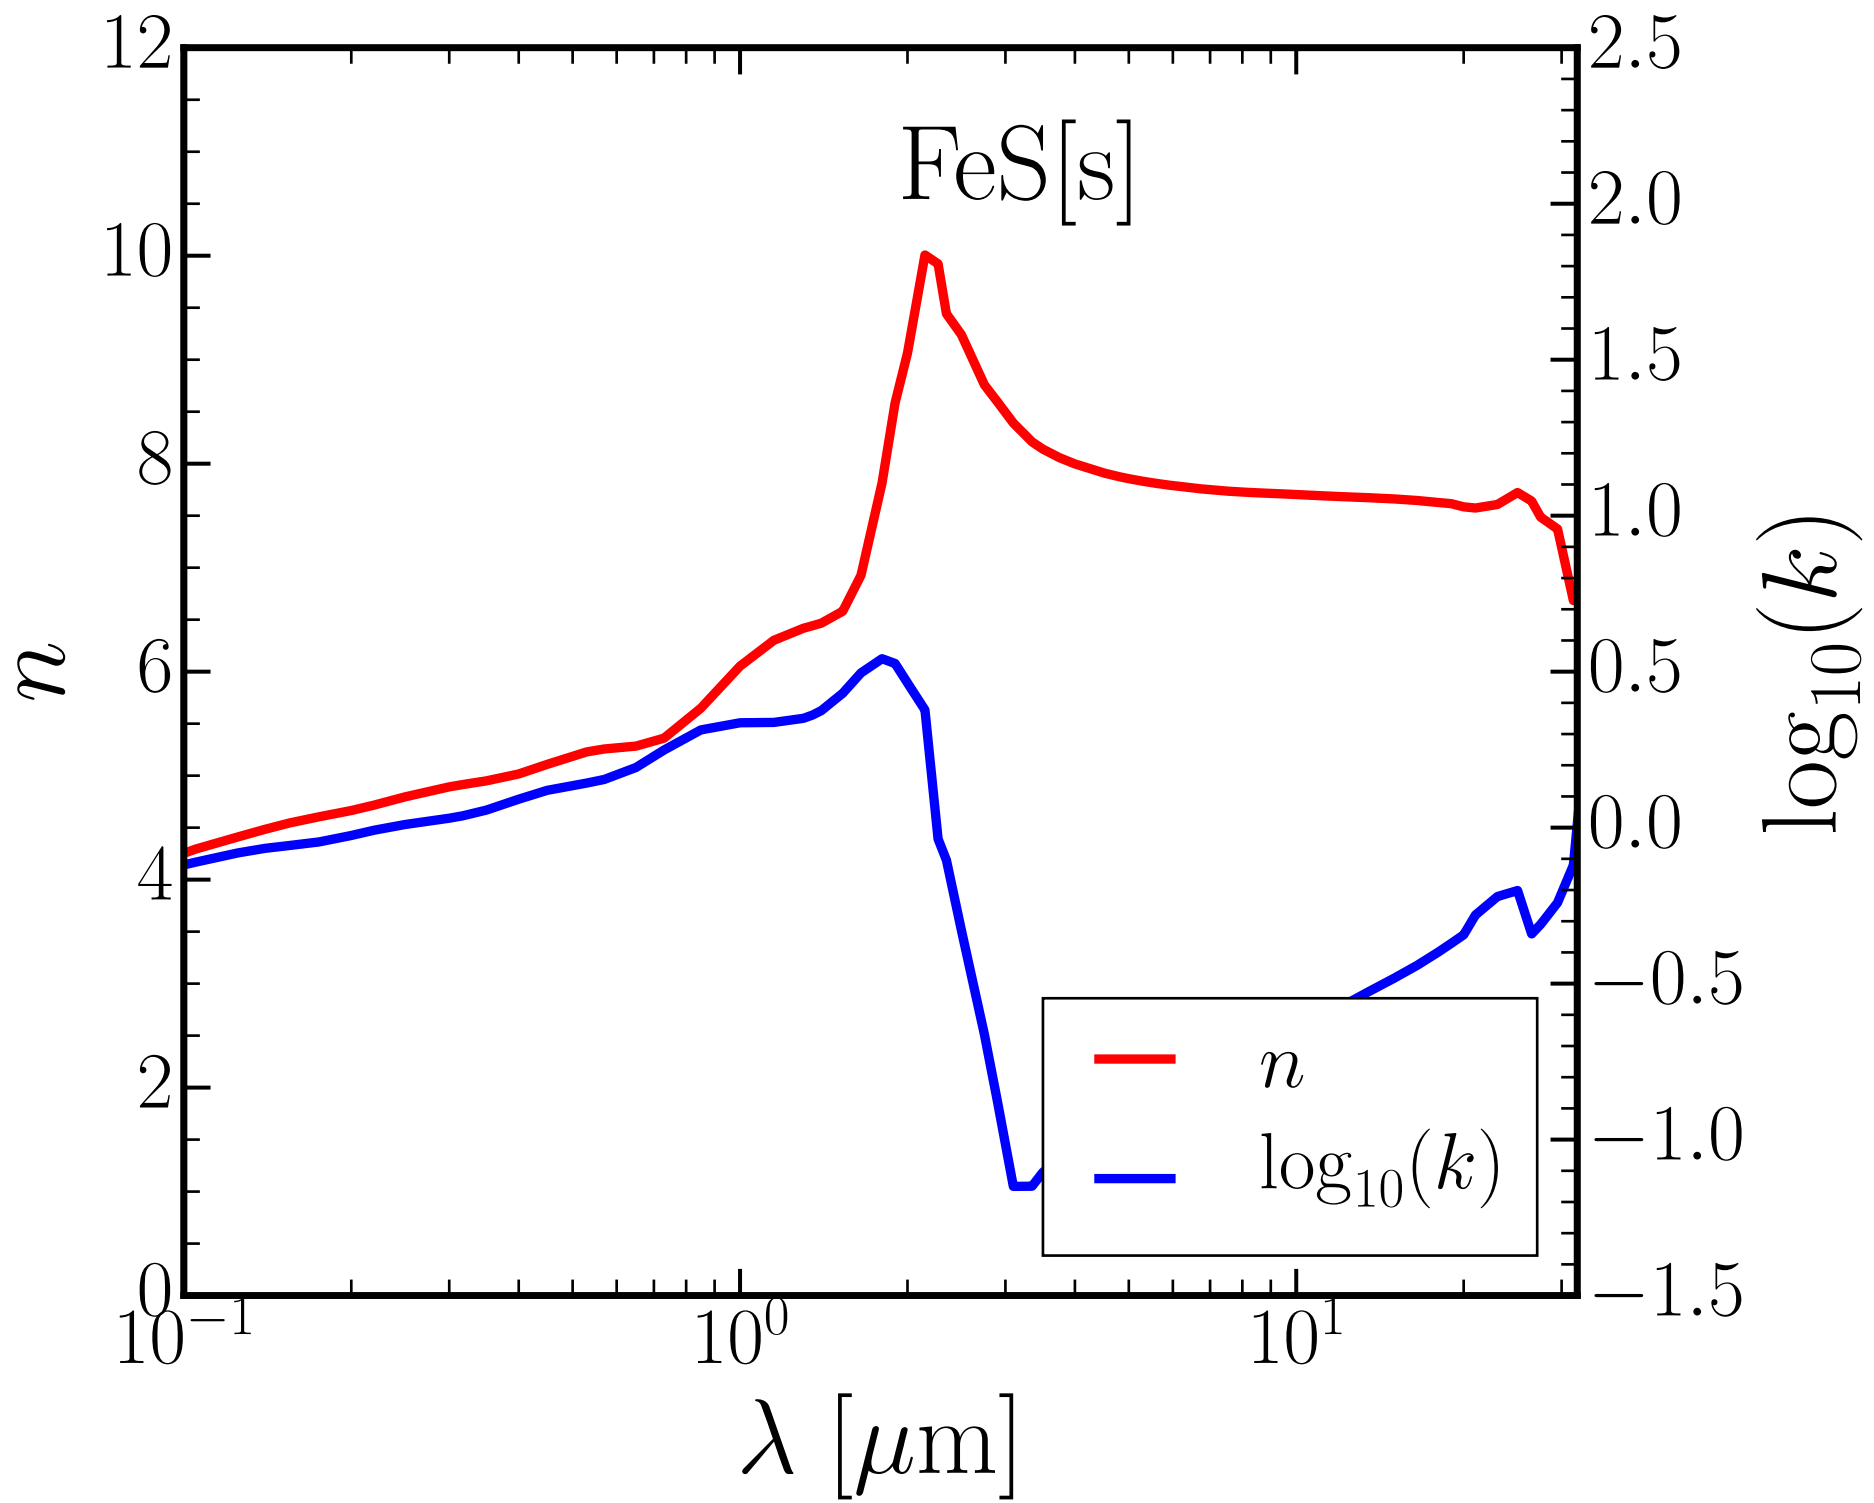

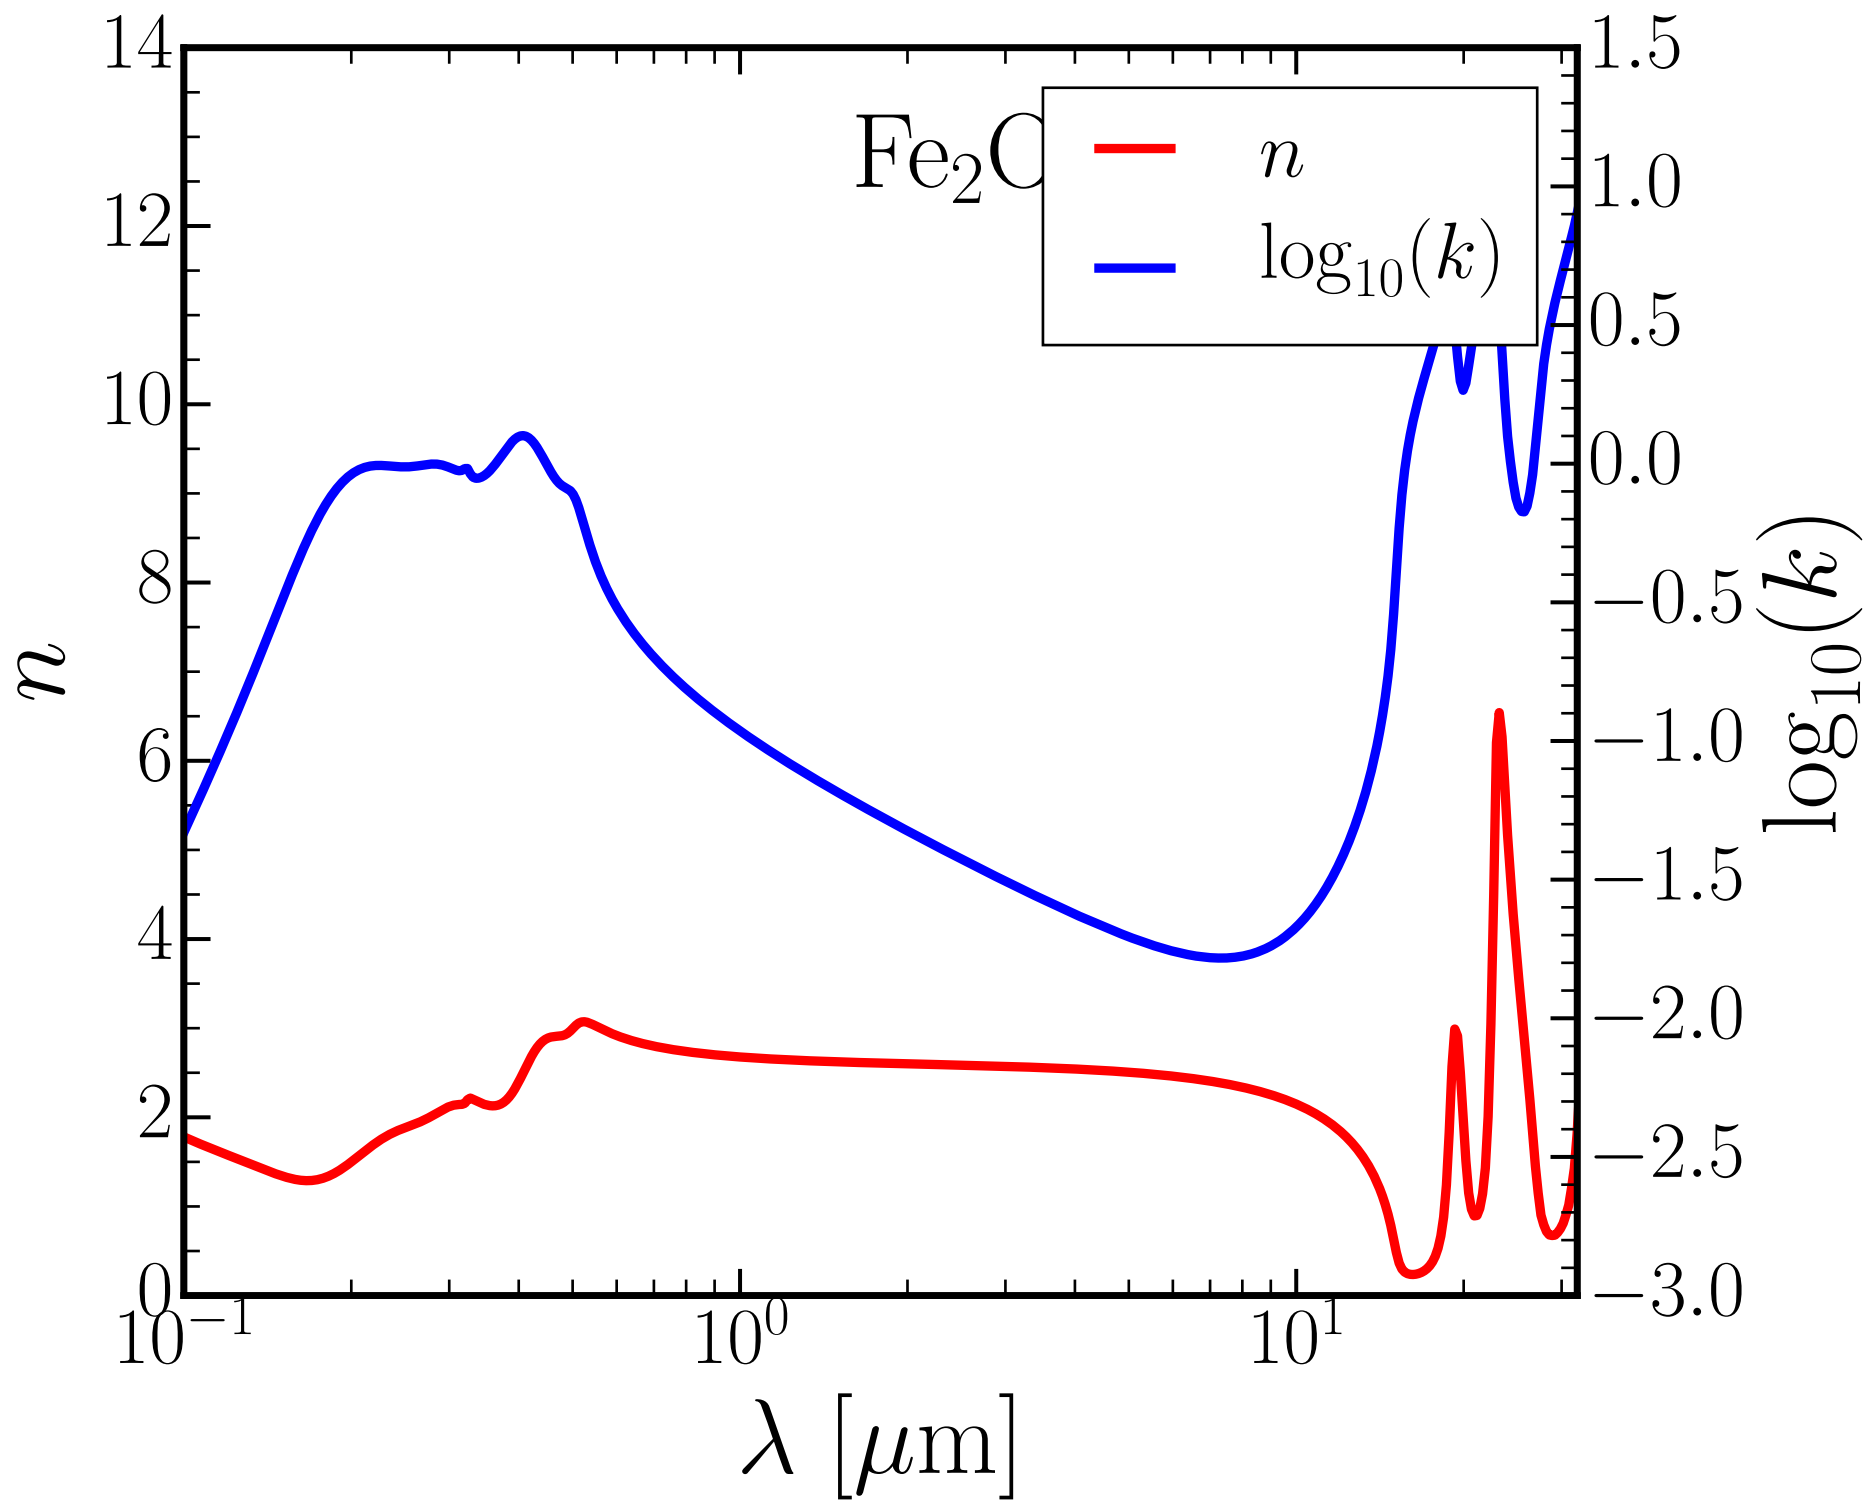

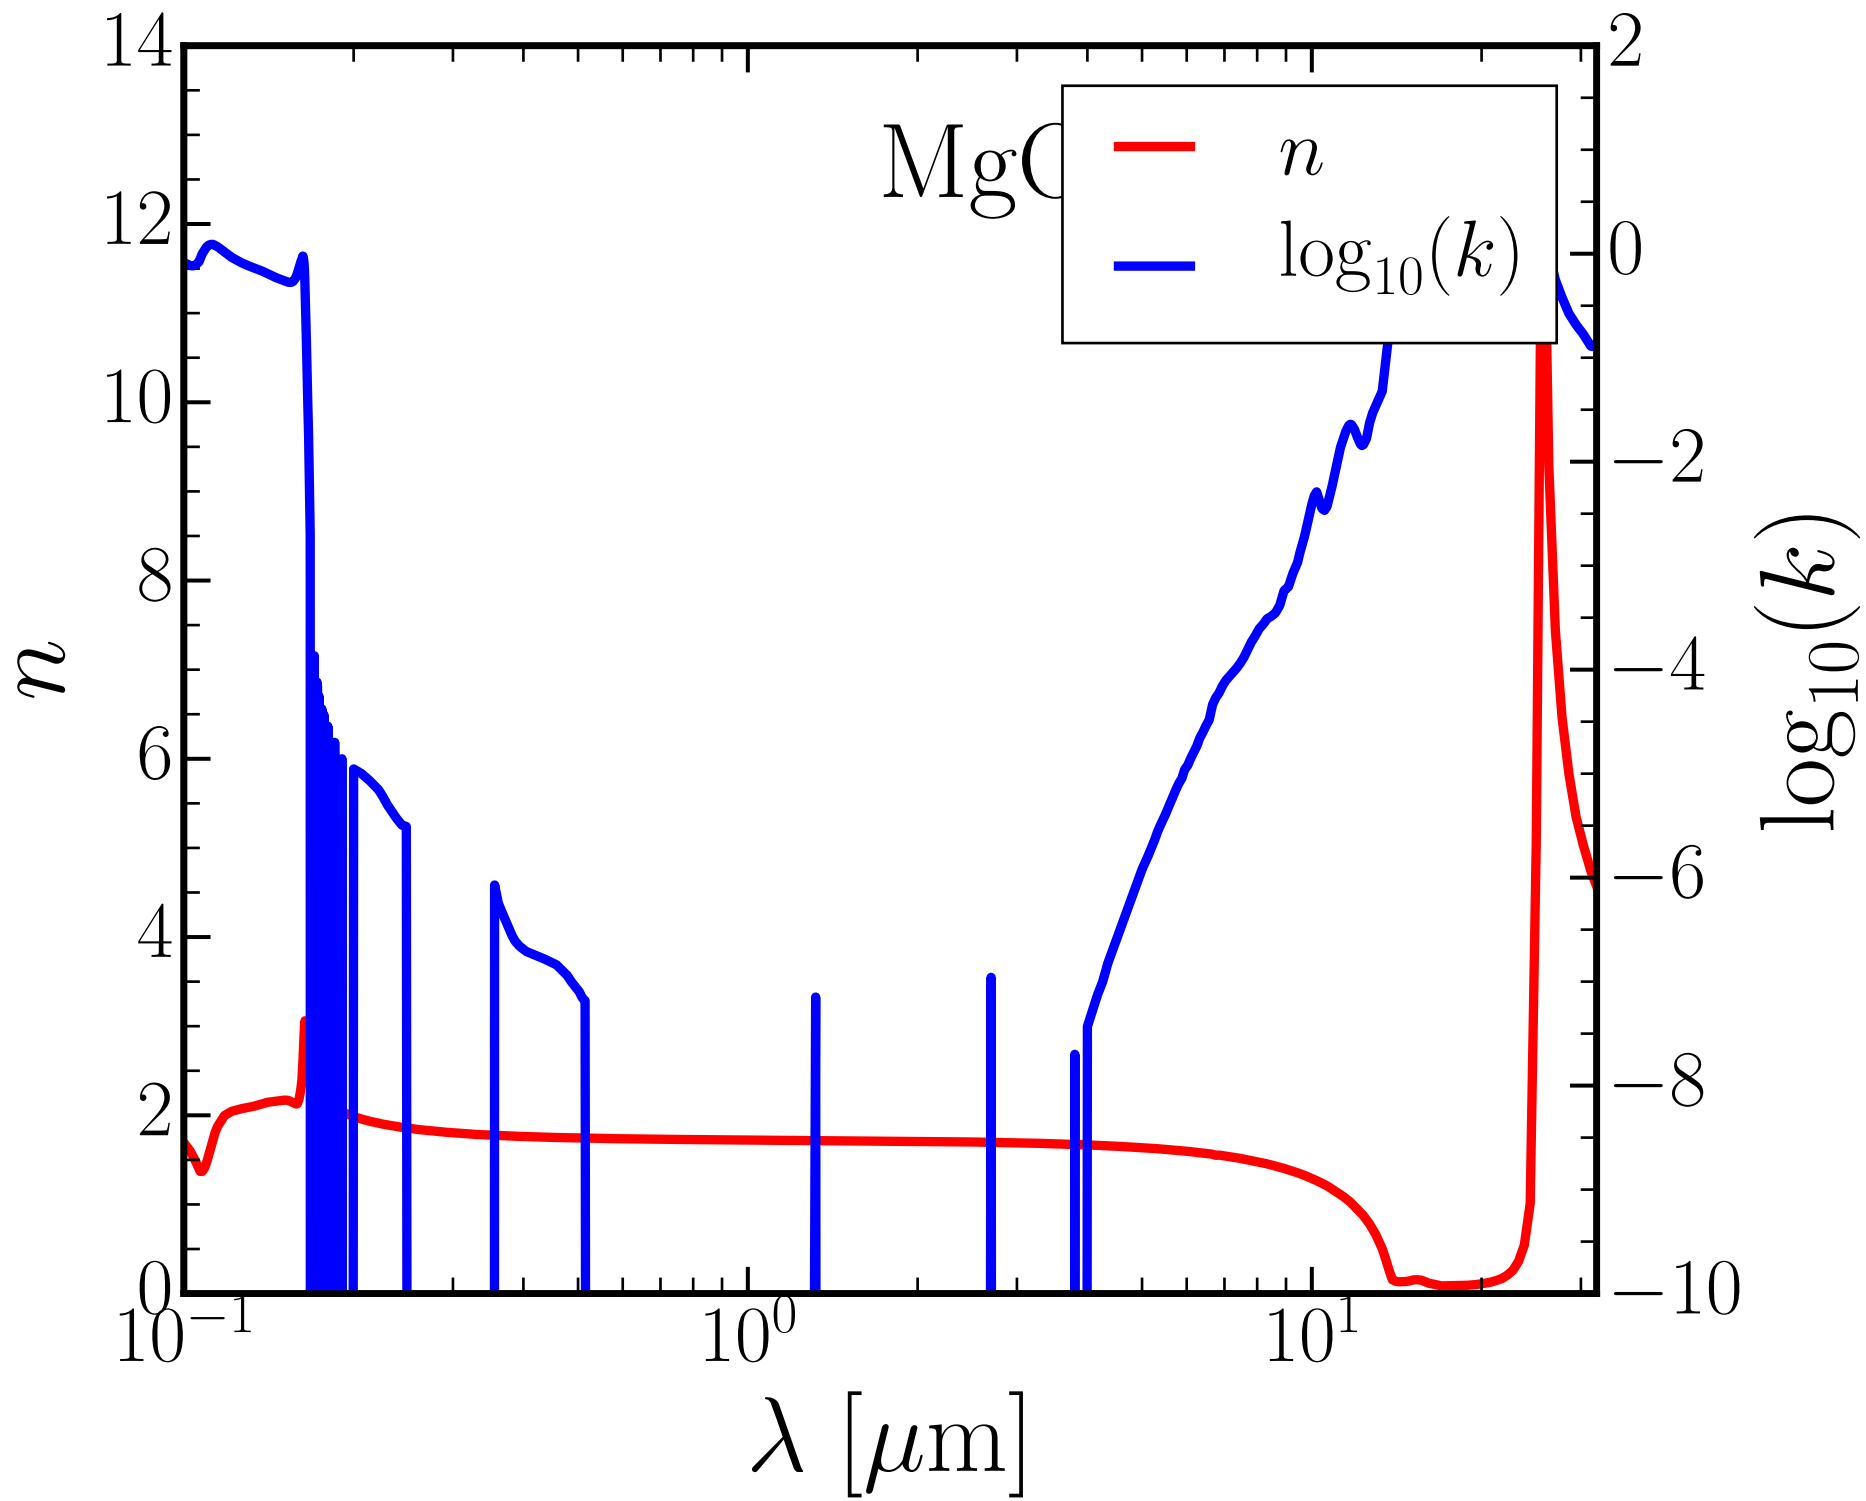

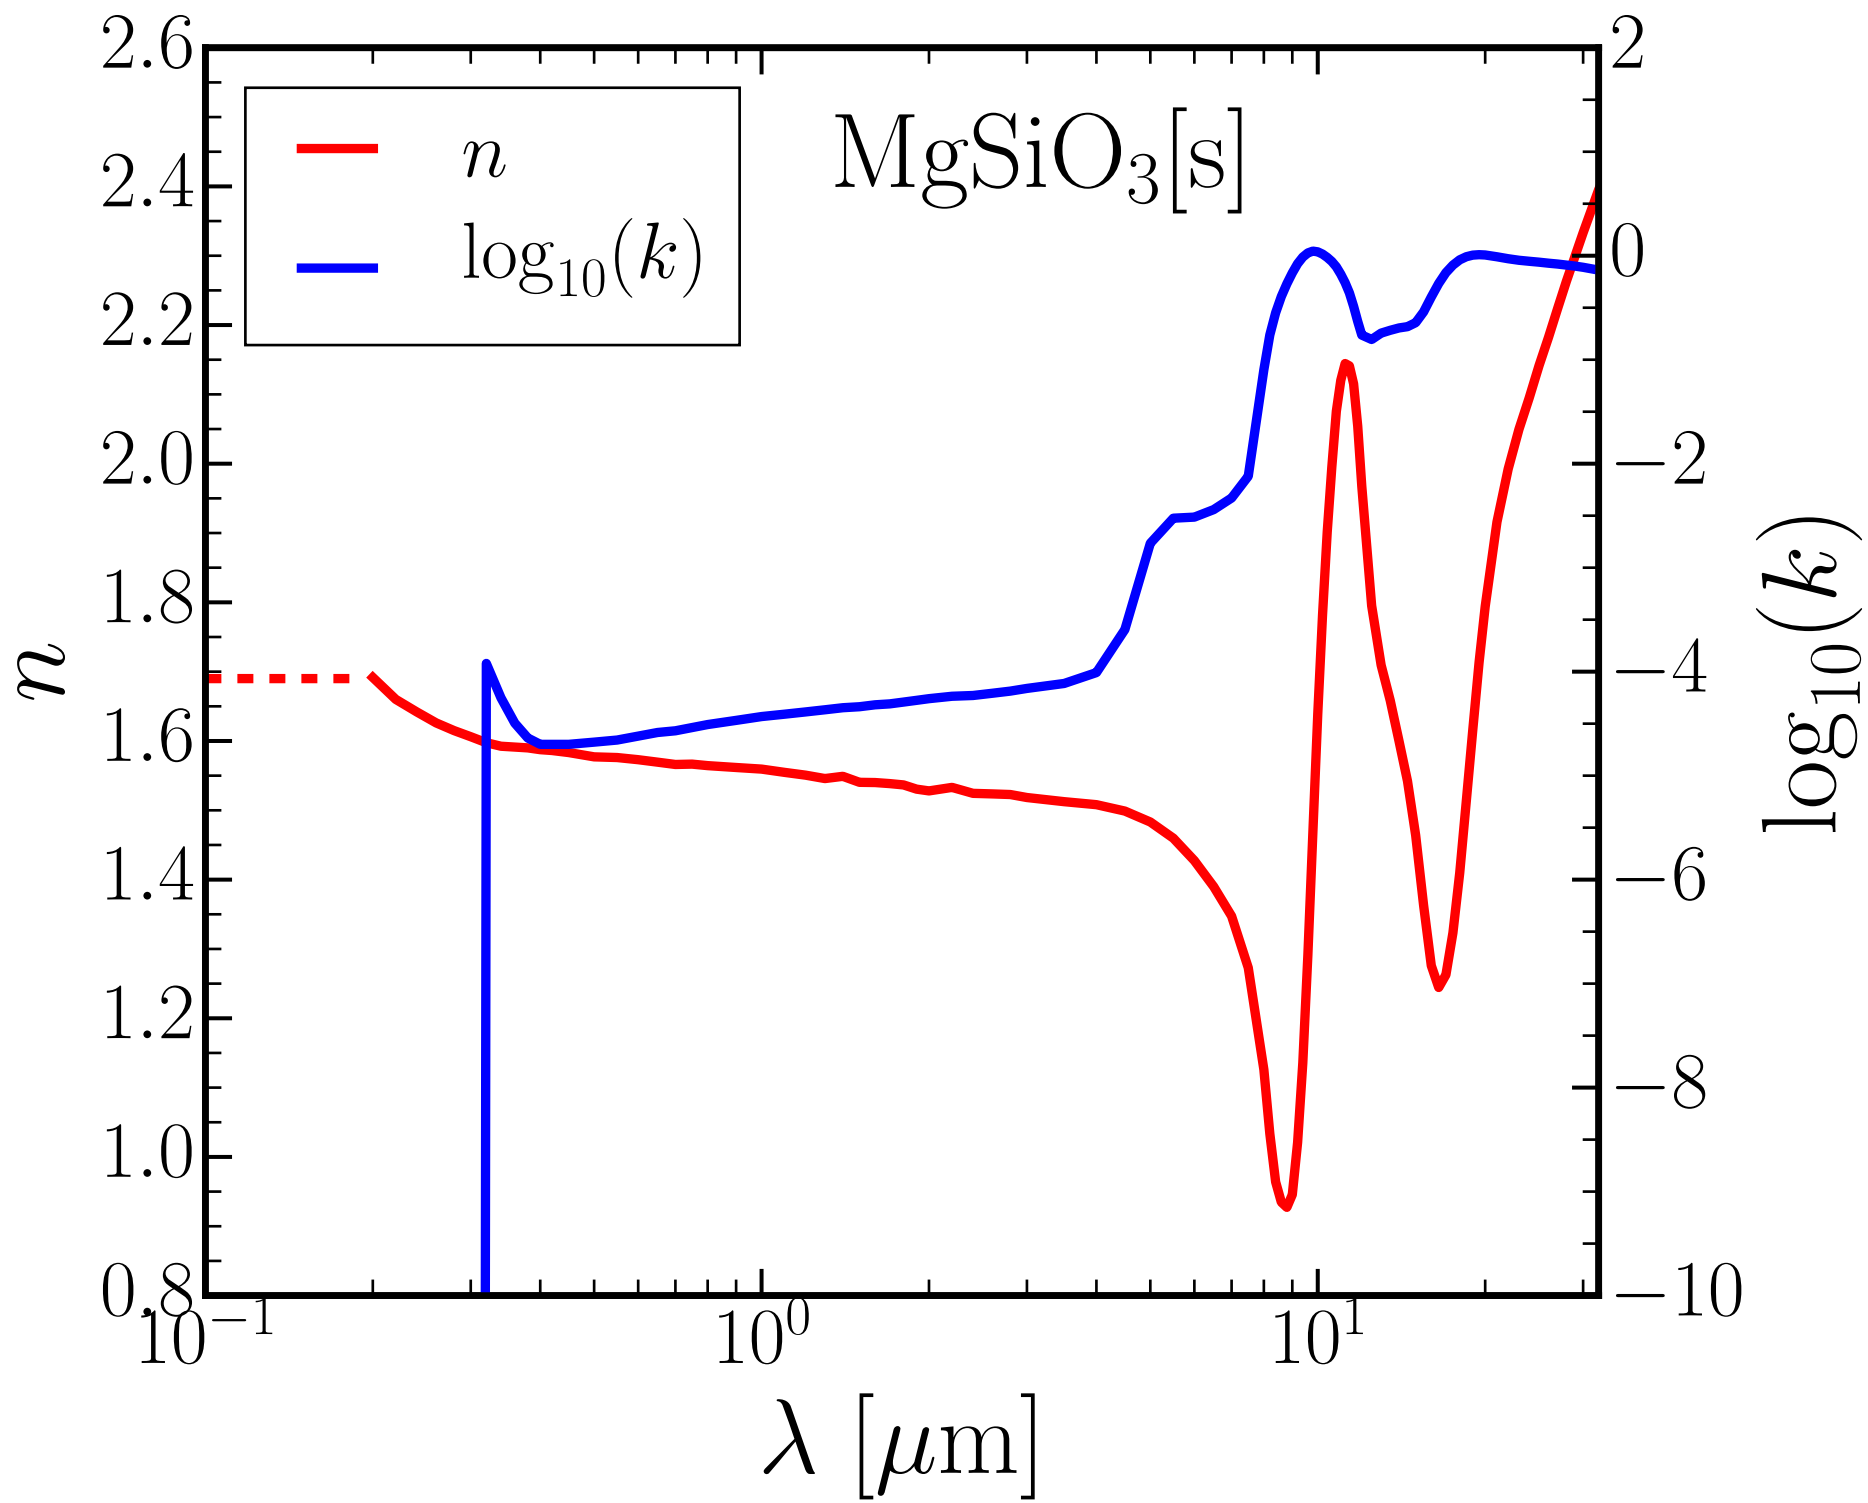

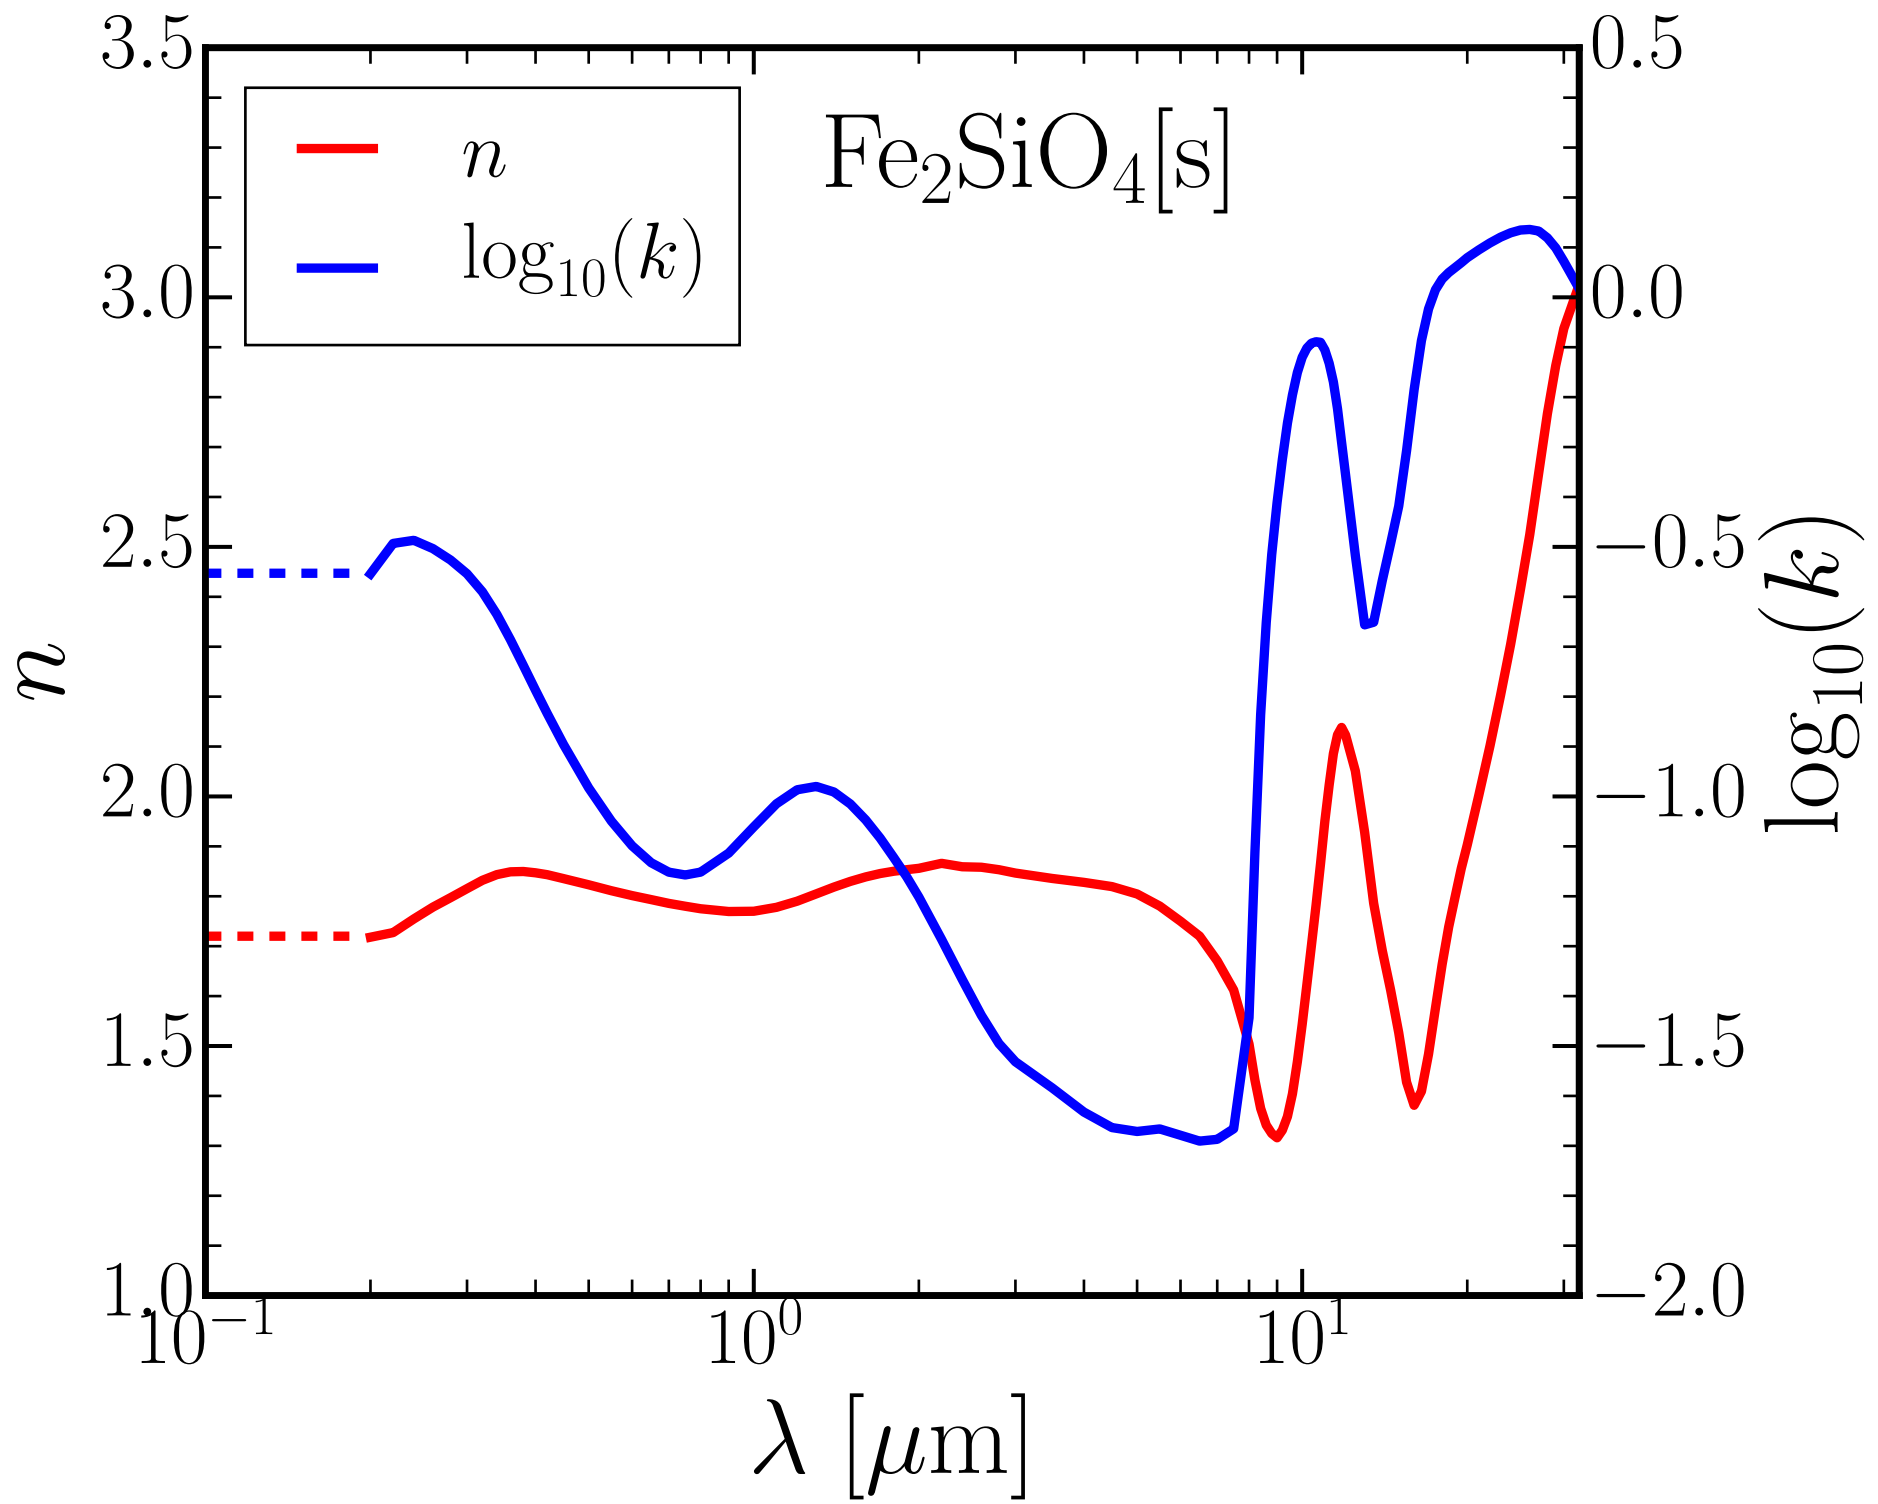

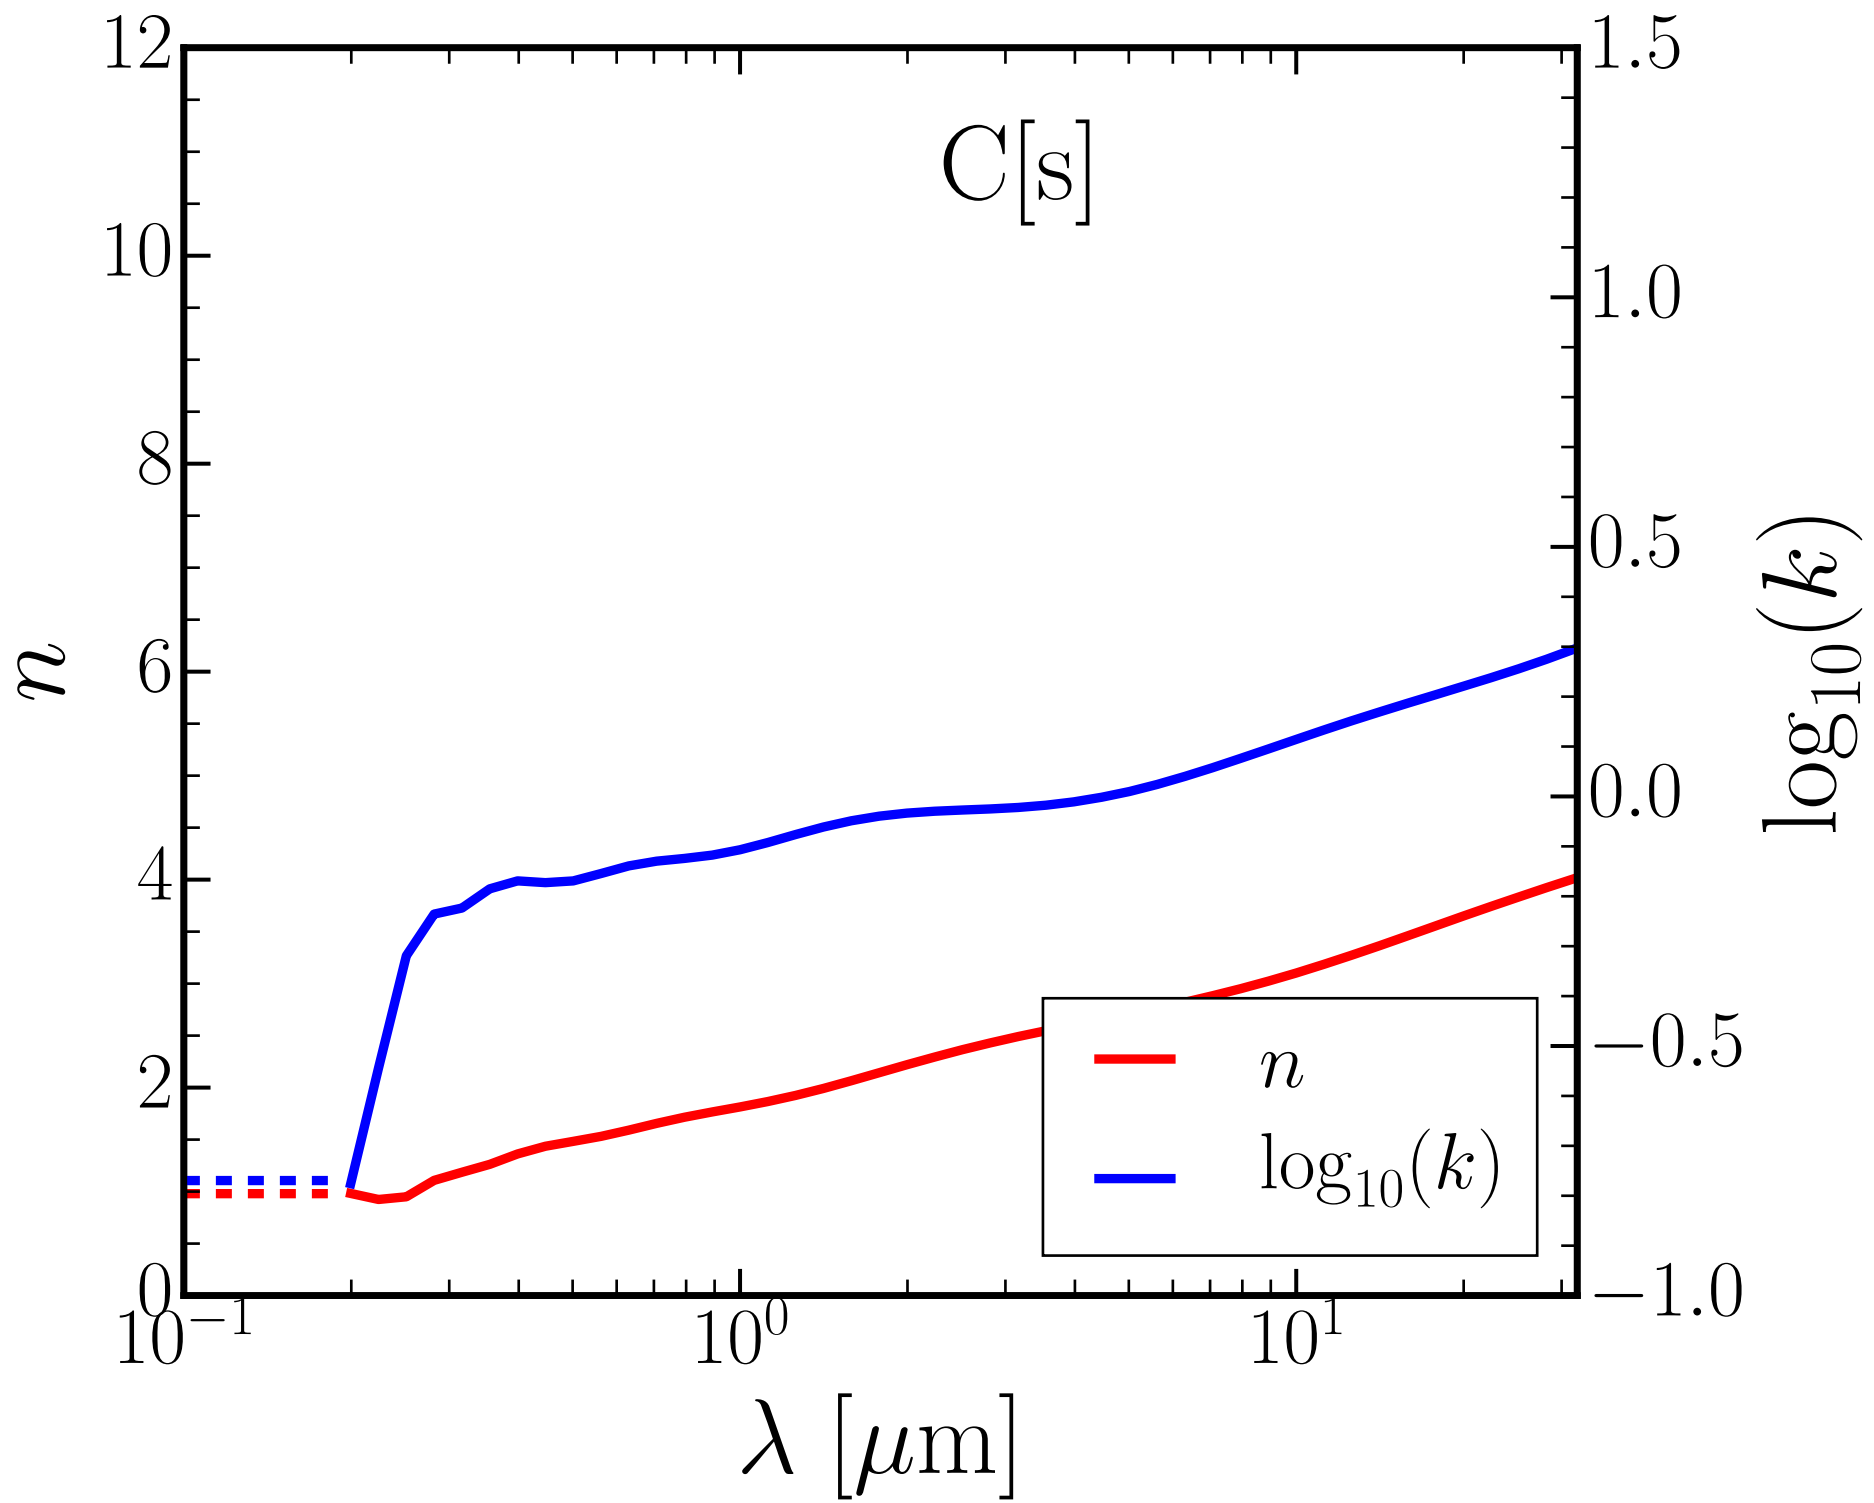

Supplement: Supplementary file 3 [file SW_Material_Refractive_Indexes_APPENDIX_logscale_32mum_labelled.pdf]
